# Supplementary material for: ExpertLongBench: Benchmarking Language Models on Expert-Level Long-Form Generation Tasks with Structured Checklists
Source: arXiv:2506.01241 source file (2025-10-07)
Supplement: Supplementary file 1 [file appendix_T09.tex]

\subsection{Task 9: Medical - Discharge Summarization} \sheza{@Sheza}\jie{jie}

\subsubsection{Task Definition}
Medical discharge summarization involves creating a structured and comprehensive summary of a patient’s hospital stay, intended to support continuity of care and communicate key clinical information to healthcare professionals and patients. Data for this task are drawn from the MIMIC-IV database \cite{johnson2024mimic}, a large publicly available dataset of deidentified electronic health records (EHRs) from critical care units.

The objective is to generate an accurate and coherent discharge summary from structured and unstructured EHR data, which includes demographics, procedures, medications, diagnoses, laboratory results, vital signs, and clinical notes of the patient. The task simulates the workflow of physicians who synthesize these inputs into formal discharge documentation.

When applying language models to this task, the input consists of EHR data (structured fields and free-text clinical notes) from a single hospital admission, and the output is a physician-style discharge summary that encapsulates the entire episode of care. An example of input data and sample human reference is available in Table \ref{tab:T9-example}.
%\jie{cite a sample figure/table here}
Human reference summaries are those originally written by physicians in the MIMIC-IV-Note dataset \cite{johnson2023mimicnote}. These summaries serve as ground truth, reflecting expert synthesis of the relevant patient data.

While prior studies have used MIMIC datasets to explore text generation in the medical domain, existing work often emphasizes extractive summarization over complex long-form text generation or lacks detailed and finegrained evaluation criteria. In contrast, our work utilizes the rich MIMIC-IV dataset, applying rigorous selection criteria and grounding the task definition in clinical documentation standards. We further extend this line of work by developing a checklist-based evaluation rubric derived from clinical best practices, specifically the Joint Commission’s discharge summary requirements \cite{kind2008documentation}, to assess the completeness and clinical relevance of generated outputs.

\subsubsection{Task Significance}
Discharge summaries are critical documents that ensure safe transitions of care, provide legal records of hospitalization, and facilitate communication between hospital teams, primary care providers, and patients. Poorly written or incomplete discharge summaries have been associated with adverse patient outcomes, such as medication errors, readmissions, and delayed follow-up care.

Automatically generating discharge summaries from EHR data can significantly reduce physician workload and documentation time, allowing clinicians to focus more on patient care. Language model-driven summarization can support more consistent and complete reporting, particularly in resource-constrained or high-throughput clinical settings.

This task advances the development of clinical language models by targeting a real-world, high-impact application that combines structured data reasoning and natural language generation. We introduce explicit selection criteria to ensure \textbf{difficulty}, \textbf{diversity}, and to objectively select complex, representative samples for the dataset.
% \jie{add objective for data selection: selecte representative samples}
Difficulty is determined through factors such as discharge summary length, number of admissions, ICU stay duration, and the complexity of diagnoses and procedures. Diversity is ensured across medication regimens, disease types, and patient demographics (age, gender, ethnicity) available in the MIMIC-IV database \cite{johnson2024mimic}. 
% \jie{add where you get these meta-data, from the original database or somewhere else} 
By framing the task with robust data, expert references, and fine-grained evaluation, this work contributes to safer, more efficient, and more interpretable clinical AI systems.

\subsubsection{Data Acquisition and Preprocessing}

We compiled data using structured patient records and discharge summaries from the MIMIC-IV (v3.1) \cite{johnson2024mimic} and MIMIC-IV-Note (v2.2) \cite{johnson2023mimicnote} datasets, hosted on PhysioNet\footnote{\url{https://physionet.org/content/mimiciv/3.1/} and \url{https://www.physionet.org/content/mimic-iv-note/2.2/}}. These datasets provide large-scale, de-identified, real-world hospital data from the Beth Israel Deaconess Medical Center.

MIMIC-IV-Note contains 331,794 discharge summaries corresponding to 145,915 unique patients. Each summary contains long-form clinical narratives written by healthcare providers at the time of hospital discharge. In parallel, we used structured tables from MIMIC-IV to retrieve metadata and clinical signals related to the patient’s hospital stay, including diagnoses, procedures, ICU stays, and medications.

We then selected a small, high-quality and representative subset from the large-scale dataset to evaluate the ability of LLMs to summarize complex patient cases. 

For representative data selection, we filtered the data based on the following standards:

\begin{itemize}
    \item \textbf{Difficulty}: We identified several factors influencing medical case complexity based on clinical expert discussions and prior literature:
    \begin{itemize}
        \item \textbf{Length of the discharge summary}: We used token count as a proxy for textual complexity, prioritizing longer summaries.
        \item \textbf{Number of hospital admissions}: Frequent admissions may indicate chronic or recurring issues.
        \item \textbf{Length of ICU stay}: Prolonged ICU stays typically correlate with more critical cases.
        \item \textbf{Number of procedures and diagnoses}: A higher count of ICD codes indicates a more medically complex case.
    \end{itemize}
    
    \item \textbf{Diversity}: To ensure a representative and generalizable set of clinical conditions, we selected discharge summaries that varied across:
    \begin{itemize}
        \item \textbf{Medication diversity}: Patients prescribed a broader spectrum of drugs.
        \item \textbf{Disease diversity}: Based on diagnosis groupings (ICD-10 code variety).
        \item \textbf{Demographic attributes}: Age, gender, and ethnicity distributions.
    \end{itemize}
\end{itemize}

We first filtered the full dataset down to 10,898 discharge summaries using these criteria. From this filtered pool, we selected the top 120 most complex cases by ranking based on discharge summary length and validating that they met multiple difficulty and diversity factors. Each selected instance of human reference summary was linked to its structured records using shared identifiers (\texttt{subject\_id} and \texttt{hadm\_id}) and manually verified for completeness. The data filtering and preprocessing pipeline is implemented in Python \sheza{upload filter.ipynb on the project github}.

\subsubsection{Illustrative Example}
The sample input for the discharge summary generation task consists of structured EHR data encompassing a patient’s hospital visit. This includes clinical information such as procedures, medications, diagnoses, laboratory results, vital signs, and physician notes. An example is shown in Table \ref{tab:T9-example}. Since the full EHR records are extensive, we only display a representative subset of the input data. As shown in Table \ref{tab:T9-example}, the sample presents detailed information from a single hospital admission, including procedure codes, medication orders, diagnostic labels, and lab test outcomes. The reference output is a physician-authored discharge summary that synthesizes this structured data into a coherent narrative. It summarizes key elements such as the hospital course, specialist consultations, performed procedures, discharge status, prescribed medications, as well as post-discharge instructions related to diet, activity, and follow-up care.

\begin{table}[!htbp]
\centering
\begin{tcolorbox}[title=Task 9-Hospital Discharge Summary: A Sample EHR Record and Summary]

\textbf{Structured EHR Input (Sample Record):}

\textbf{Note ID:} 14767018-DS-20 \\
\textbf{Subject ID:} 14767018 \\
\textbf{HADM ID:} 21575486 \\
\textbf{Note Type:} DS (Discharge Summary) \\
\textbf{Chart Time:} 2156-07-27 00:00:00 \\
\textbf{Store Time:} 2156-07-27 21:46:00 \\
\textbf{Diagnoses (ICD-10)}  
\begin{itemize}
  \item Sepsis, unspecified organism (A419)
  \item Acute kidney failure with tubular necrosis (N170)
  \item Acute and subacute hepatic failure without coma (K7200)
  \item Acute respiratory distress syndrome (J80)
  \item Severe sepsis with septic shock (R6521)
  \item Pneumonia, unspecified organism (J189)
  \item Other sites of candidiasis (B3789)
  \item Chronic pulmonary edema (J811)
  \item Thrombosis due to vascular prosthetic devices, initial encounter (T82868A)
  \item Delirium due to known physiological condition (F05)...
\end{itemize} 
\textbf{Procedures (ICD-10-PCS)} 
\begin{itemize}
  \item Respiratory Ventilation, >96 Consecutive Hours (5A1955Z)
  \item Urinary Filtration, Multiple (5A1D60Z)
  \item Nutritional Substance to Upper GI, Via Opening (3E0G76Z)
  \item Infusion Device into Right Internal Jugular Vein (05HM33Z)
  \item Echocardiography (B543ZZA)*...
\end{itemize} 
\textbf{Drugs Administered} 
\begin{itemize}
  \item 5\% Dextrose (250 mL, IV)
  \item Heparin Sodium (25,000 unit Premix Bag, IV)...
\end{itemize} 
\textbf{Patient Summary (Human-written Reference):}\\
Name: \_\_\_ Unit No: \_\_\_ Admission Date: \_\_\_ Discharge Date: \_\_\_ Date of Birth: \_\_\_ Sex: F Service: MEDICINE\\
Allergies:
cefepime\\
Attending: \_\_\_.\\
Chief Complaint:
Acute hypoxemic respiratory failure\\
Major Surgical or Invasive Procedure:
intubation, bronchoscopy, extubation, LIJ, right tunneled HD line, HD\\
History of Present Illness:
Ms. \_\_\_ is a \_\_\_ year old woman with history of HTN, HLD, DM2 who presents from \_\_\_ with ARDS, acute liver injury, acute renal failure. According to her husband she was previously healthy, running half marathons, has had decline in health over past several years. She has had intermittent fatigue, joint pain, cough with intermittent paroxysmal episodes resulting in vomiting. She was being treated by a homeopathic healer for chronic lyme disease, taking at least 5 homeopathic medications. She has also had recurrent sinus infections, pneumonias. She was last treated for pneumonia Labor \_\_\_.  Patient initially presented \_\_\_ to \_\_\_ with complaints of weakness, lightheadedness, lower extremity edema. On presentation there she was found to have liver failure (reported transaminases in the thousands) and concern for obstructed biliary system. ERCP showed sludge. She underwent percutaneous cholecystostomy tube placement with concern for cholecystitis...\\
\end{tcolorbox}
\caption{Task 9-Hospital Discharge Summary: A Sample EHR Record and Corresponding Summary. The "\_\_\_" indicates anonymized fields such as patient identifiers or facility names that have been removed to protect privacy in the database. 
% \jie{describe what \_\_\_ mean}
}
\label{tab:T9-example}
\end{table}

\subsubsection{Evaluation Rubric}
To evaluate the completeness and quality of discharge summaries, we designed a checklist-based evaluation rubric grounded in documentation standards published by the Joint Commission. Specifically, we follow the criteria outlined in the Joint Commission’s discharge summary content requirements, as detailed by Kind and Smith in their report on documentation quality during transitions from acute to subacute care \cite{kind2008documentation}.

This rubric consists of 12 checklist items that reflect the mandated components required for effective discharge communication. Several items are marked as 'if applicable', meaning they should be included only when clinically relevant to the patient’s case. The checklist enables standardized assessment of both the presence and quality of information in discharge documentation.

The full checklist items are as follows:

\begin{itemize} \item \textbf{Chief Complaint}: A clear statement identifying the primary reason for admission (e.g., “Patient admitted due to severe chest pain and shortness of breath”).

\item \textbf{History of Present Illness}: A concise summary of the patient’s presenting symptoms and their clinical progression (e.g., “A 58-year-old male with a history of hypertension presented with acute onset chest pain radiating to the left arm”).

\item \textbf{Primary Diagnosis}: The admission and discharge diagnoses should be explicitly documented (e.g., “Final diagnosis: Acute Myocardial Infarction”).

\item \textbf{Hospital Course}: A chronological overview of the clinical management and significant events during hospitalization (e.g., “Patient was started on heparin drip, underwent cardiac catheterization on Day 2”).

\item \textbf{Consultations} (if applicable): Documentation of any specialty consultations received (e.g., “Cardiology consult obtained for further evaluation of coronary artery disease”).

\item \textbf{Hospital Procedures} (if applicable): A list of diagnostic or therapeutic procedures conducted during the hospital stay (e.g., “Coronary angioplasty performed successfully”).

\item \textbf{Status at Discharge}: A brief statement describing the patient's condition at discharge (e.g., “Patient discharged in stable condition with no signs of distress”).

\item \textbf{Discharge Medications} (if applicable): A complete and updated list of prescribed medications upon discharge, including new, continued, and discontinued medications (e.g., “New prescriptions: Atorvastatin 40mg, Clopidogrel 75mg”).

\item \textbf{Activity Instructions} (if applicable): Specific recommendations or restrictions regarding physical activity (e.g., “Patient advised to avoid strenuous exercise for 2 weeks”).

\item \textbf{Therapy Orders} (if applicable): Instructions for physical, occupational, or speech therapy, if relevant (e.g., “Referral to outpatient cardiac rehab scheduled”).

\item \textbf{Dietary Instructions} (if applicable): Nutritional guidance tailored to the patient’s clinical condition (e.g., “Low-sodium, heart-healthy diet recommended”).

\item \textbf{Follow-up Appointments} (if applicable): Scheduled follow-up visits and provider contact details (e.g., “Follow-up with cardiologist in one week”). \end{itemize}

This evaluation framework ensures that discharge summaries are assessed for their alignment with clinical standards required for safe transitions of care and continuity across healthcare settings.

\subsubsection{Checklist-mapped Reference}
% example ref needs to be changed, this is an older one - setting as placeholder here

To assess model performance in generating discharge summaries aligned with critical clinical information needs, we construct checklist-mapped references that extract content corresponding to each checklist item from the original discharge summary using GPT-4o. An illustrative example of this process is shown in Table \ref{tab:T9-Checklist-mappedReference}. For each checklist item, we carefully follow its formal definition and prompt the model to extract the most relevant content from the discharge summary text.

Similar to our approach in Task 1, we adopt a role-playing prompt in which the model is instructed to act as a medical assistant tasked with extracting essential clinical information. If the information is not explicitly available in the summary, the model is instructed to return "N/A". To ensure efficiency and consistency, we group the checklist items based on content type and expected length, allowing multiple extractions within a single prompt. The example prompt used for this extraction is provided in Table \ref{tab:T9-checklist-mappedReference-prompt}.
\begin{table}[!htbp] \centering \begin{tcolorbox}[title=Task 9-Hospital Discharge Summary: Checklist-mapped reference] \begin{itemize}

\item \textbf{Chief Complaint}: Transfer from OSH for HRS and liver transplant workup.

\item \textbf{History of Present Illness}: Mr. \underline{\hspace{3cm}} is a \underline{\hspace{3cm}} man with EtOH cirrhosis complicated by portal hypertension/ascites, history of subtotal colectomy for UC and colectomy for dysplasia/bleeding with post-op course complicated by decompensated portal hypertension, presenting with jaundice and pruritis. He had been doing well since his colectomy last year with ascites well controlled on diuretics. He began to experience itching several weeks before presentation. His family noticed jaundice and pruritis during a holiday visit, prompting him to see his PCP. Labs at the PCP visit showed elevated bilirubin (21) and creatinine (2.7). He was subsequently admitted to OSH and later transferred for further evaluation and liver transplant workup.

\item \textbf{Primary Diagnosis}: ETOH Cirrhosis, decompensated s/p liver transplant.

\item \textbf{Consultations}: Nephrology for renal failure and CRRT; Cardiology for atrial fibrillation and SVTs; Psychiatry for depression and delirium; Neurology for altered mental status; Infectious Disease for VRE bacteremia and MDR E. coli; Interventional Pulmonology for pleural effusions and empyema; Thoracic Surgery for empyema management; Geriatric Medicine for delirium management.

\item \textbf{Hospital Course}: The patient underwent a deceased donor liver transplant complicated by left rib fractures, takeback for re-exploration and control of bleeding, delayed abdominal closure with small bowel resection, diminished hepatic artery blood flow requiring splenic artery embolization, and biliary anastomotic stricture requiring ERCP and stent placement. His course was further complicated by altered mental status, cardiac arrhythmias (SVTs), persistent hypotension requiring pressors, respiratory failure with bilateral pleural effusions requiring chest tube drainage, multiple enterocutaneous fistulas, renal failure requiring CRRT/HD, hypothyroidism, adrenal insufficiency, and enterococcus bacteremia. He required multiple ICU admissions and extensive multidisciplinary care.

\item \textbf{Hospital Procedures}: Deceased donor liver transplant, re-exploration for bleeding, small bowel resection, splenic artery embolization, ERCP with stent placement, left thoracentesis, chest tube placements, right VATS pleural washout, percutaneous tracheostomy, right Eloesser flap, abdominal wound debridement, liver biopsy, and multiple abdominal washouts.

\item \textbf{Status at Discharge}: Expired.

\item \textbf{Discharge Medications}: 1. Albuterol 0.083\% Neb Soln Q6H PRN, 2. Dextrose 50\% IV PRN, 3. Ganciclovir 60 mg IV post-HD, 4. Glucagon 1 mg IM PRN, 5. Glucose Gel 15 g PO PRN, 6. Heparin 5000 UNIT SC BID, 7. HYDROmorphone 0.125-0.25 mg IV PRN, 8. Hydromorphone Oral Solution 1 mg/mL Q4H PRN, 9. Ipratropium Bromide Neb Q6H PRN, 10. Ipratropium-Albuterol Neb Q6H, 11. MethylPREDNISolone 4 mg IV Q24H, 12. Midodrine 10 mg PO TID, 13. Mycophenolate Mofetil 1000 mg IV BID, 14. Neomycin-Polymyxin-Bacitracin PRN, 15. Pantoprazole 40 mg IV Q12H, 16. Sarna Lotion QID PRN, 17. Sodium Chloride Nasal Spray QID PRN, 18. Sodium Polystyrene Sulfonate 15 gm PO PRN, 19. Sulfameth/Trimethoprim SS 1 TAB PO DAILY, 20. Tacrolimus 0.5 mg and 1 mg PO BID, 21. TraZODone 50 mg PO QHS.

\item \textbf{Activity Orders}: Out of bed with assistance to chair or wheelchair. No driving if taking narcotic pain medications.

\item \textbf{Therapy Orders}: N/A

\item \textbf{Dietary Instructions}: Eat small frequent meals, supplement with Carnation Instant Breakfast or Ensure. Avoid direct sun exposure and drink enough fluids to keep urine light in color.

\item \textbf{Follow-up Appointments}: Follow up with the transplant clinic. Labwork to be drawn twice weekly as arranged by the transplant clinic.

\end{itemize} \end{tcolorbox} \caption{Task 9-Hospital Discharge Summary: Checklist-mapped reference.} \label{tab:T9-Checklist-mappedReference} \end{table}
\begin{table}[!htbp]
\centering
\begin{tcolorbox}[title=Task 9 - Hospital Discharge Summary: Prompt for extracting checklist-mapped reference, colback = yellow!5]

You are a medical professional extracting key clinical information from a hospital discharge summary. Given a discharge summary, extract:

\begin{enumerate}
    \item \textbf{Chief Complaint} – The main reason the patient was admitted to the hospital. Include associated symptoms and context, such as “presented with,” “admitted for,” etc.
    
    \item \textbf{History of Present Illness} – The timeline and progression of symptoms before admission. Include relevant medical, surgical, family, or social history, allergies linked to the complaint, and any patient-reported events or treatments prior to admission.
    
    \item \textbf{Primary Diagnosis} – The primary diagnosis at both admission and discharge. Include confirmed diseases, conditions, or syndromes. If multiple diagnoses are mentioned, extract the most emphasized one.
    
    \item \textbf{Consultations} – Any specialist consults requested during the stay. Include the specialty (e.g., cardiology), reason for consult, and recommendations or findings.
    
    \item \textbf{Hospital Course} – A summary of the clinical course during the hospital stay, including major events, complications, tests, clinical exams, and medical decision-making.
    
    \item \textbf{Hospital Procedures} – Diagnostic, surgical, or therapeutic procedures conducted. Include names, purposes, and results if mentioned.
    
    \item \textbf{Status and Disposition at Discharge} – The patient’s condition at discharge: symptom resolution, clinical stability, functional status, or changes since admission.
    
    \item \textbf{Discharge Medications and Instructions} – Prescribed medications and instructions at discharge. Include drug names, dosages, routes (e.g., oral, IV), and frequencies (e.g., once daily, BID).
    
    \item \textbf{Activity Orders} – Any physical activity-related instructions, such as walking or lifting restrictions.
    
    \item \textbf{Therapy Orders} – Physical, occupational, or speech therapy recommended post-discharge, with specified goals if given.
    
    \item \textbf{Dietary Instructions} – Any dietary restrictions or advice, such as diabetic diets or food restrictions.
    
    \item \textbf{Follow-up Appointments} – Recommended follow-up visits including specialty, reason, and timing (e.g., “follow up with cardiology in 2 weeks”).
\end{enumerate}

Extract all fields as thoroughly as possible. If a field is missing or not mentioned, return "N/A" (as a string). Do not make assumptions beyond the text. 

\textbf{Output format (all values must be strings, no arrays or nested structures):}

\begin{verbatim}
{
  "Chief Complaint": "string",
  "History of Present Illness": "string",
  "Primary Diagnosis": "string",
  "Consultations": "string",
  "Hospital Course": "string",
  "Hospital Procedures": "string",
  "Status at Discharge": "string",
  "Discharge Medications": "string",
  "Activity Orders": "string",
  "Therapy Orders": "string",
  "Dietary Instructions": "string",
  "Follow-up Appointments": "string"
}
\end{verbatim}

This is the discharge summary:

\end{tcolorbox}
\caption{Task 9 - Hospital Discharge Summary: Prompt for extracting checklist-mapped reference.}
\label{tab:T9-checklist-mappedReference-prompt}
\end{table}

As part of our quality control process, we manually evaluated the checklist-mapped references from 30 challenging and diverse discharge summaries sampled from the broader dataset. Evaluators assessed the extractions for faithfulness to the source text. 
%and we additionally used GPT-based models such as Gemini and Claude to perform automated assessments of faithfulness and coverage. \sheza{To be updated with human and model evaluation details, prompts, results, and conclusion.} \jie{we may not use GPT-based models such as Gemini and Claude to do automatic assessments of this task}
