# Supplementary material for: ExpertLongBench: Benchmarking Language Models on Expert-Level Long-Form Generation Tasks with Structured Checklists
Source: arXiv:2506.01241 source file (2025-10-07)
Supplement: Supplementary file 2 [file appendix_J_use_of_LLMs.tex]

{

\section{The Use of Large Language Models}
\label{ap:useofllm}
In this work, large language models were primarily employed to assist in polishing the manuscript's language and grammar. Their use was limited to improving readability, ensuring linguistic correctness, and maintaining a formal academic tone, without altering the scientific content or interpretation of the results.
}
