# Supplementary material for: ExpertLongBench: Benchmarking Language Models on Expert-Level Long-Form Generation Tasks with Structured Checklists
Source: arXiv:2506.01241 source file (2025-10-07)
Supplement: Supplementary file 3 [file appendix.tex]

\appendix

\newlist{todolist}{itemize}{2}
\setlist[todolist]{label=$\square$}

\section{Task Description}
\sheza{review task descriptions}

\subsection{Task 1: Legal - Case Summarization}
\jie{@jie}
\subsubsection{Task Definition}
% \lu{we should cite this paper https://multilexsum.github.io/, since they do the same task, then say this work collects new data and create checklist, etc. basically note the difference}\jie{have added a paragraph to discuss the difference, move it to the 'Task Significance' Section as we better description the task on civil rights litigation in that section}
Legal case summarization involves generating concise, coherent, and informative summaries from multiple legal documents pertaining to a single case. 
These documents can include a wide range of materials such as complaints, appeals, court opinions, motions, filings, judgments, and other related legal records.
The \textbf{objective} is to summarize critical aspects of a case into a summary that is accessible to a broad audience, including legal professionals such as policymakers, advocates, researchers, educators, and students, as well as the general public. A sample summary is displayed in Figure \ref{tab:T1-example}.
When using LLM to conduct the legal case summarization task, the input is typically a collection of relevant legal documents associated with a specific case and the output is a case summary that encapsulates the essential information from the original documents.


\subsubsection{Task Significance}
% \lu{this paragraph is ok, but sounds very high level, you can take a look at clearinghouse website, and see if they give any motivation, or check the documents shared by Margo's team}\jie{have updated one version}
Legal case summarization is a foundational task for improving access to justice, supporting legal research, and facilitating informed decision-making across the legal system. Many real-world cases involve large volumes of interrelated documents. These include complaints, motions, rulings, and settlement agreements, which must be synthesized into concise, coherent summaries.
Automatic summarization addresses this issue by condensing lengthy texts into concise summaries, enabling users to quickly grasp essential details without reading the entire document \cite{shen2022multi}. This automation enhances accessibility by providing clear summaries for lawyers, scholars, and the general public, improves efficiency by assisting legal professionals in quickly understanding case details, and supports research by highlighting crucial aspects of cases. By reducing the time and effort required to comprehend extensive legal materials from legal experts, automatically generated summaries streamlines legal workflows and aids in informed decision-making. This challenge becomes even more pronounced in domains where litigation is prolonged, procedurally complex, and socially impactful.

One such domain is civil rights litigation, which has played a pivotal role in reforming public institutions and shaping policy in areas such as education, policing, incarceration, and disability rights. These cases often span years and generate hundreds of filings, yet most remain inaccessible to the broader public, scholars, and even practitioners. The Civil Rights Litigation Clearinghouse\footnote{\url{https://clearinghouse.net/}}, a leading repository in this space, curates extensive documentation from landmark and ongoing civil rights cases—many of which have never resulted in published judicial opinions. As a result, key legal developments are often buried in fragmented, unstructured documents that are difficult to access and interpret without expert knowledge. Multi-document case summarization helps bridge the accessibility gap. It enables non-experts to understand legal developments, allows legal professionals to quickly grasp the structure and outcome of complex cases, supports advocacy and policymaking by surfacing systemic patterns, and reduces the burden of reviewing lengthy legal documents, giving researchers easier access to representative case content. We collect data from Clearinghouse, with further details provided in Section \ref{ap:sec-T1-dataAcquisition}.
% \lu{after such a long introduction of clearinghous, you should say we collect data from this initiative which is described in the next section}


A related work, Multi-LexSum \cite{shen2022multi}, also investigates the task of multi-document legal case summarization in civil rights litigation domain using data from the Clearinghouse. However, their study primarily relies on automatic evaluation metrics such as ROUGE-\{1,2,L\} \cite{lin2004rouge} and BERTScore \cite{zhang2019bertscore}. 
In contrast, our work constructs a new dataset by collecting cases data from the Clearinghouse and introducing clear selection criteria with legal researchers grounded in both \textbf{diversity} and \textbf{difficulty}, where diversity refers to the range of case topics and difficulty is based on structural factors such as such as the number of documents, length, and complexity of legal proceedings.
Furthermore, we develop a fine-grained, checklist-based evaluation rubric in collaboration with a legal researcher to ensure comprehensive coverage of key case elements. To assess model performance more reliably, we design a structured evaluation pipeline leveraging LLMs as evaluators, enabling nuanced analysis beyond surface-level lexical similarity.
\subsubsection{Data Acquisition and Preprocessing}\label{ap:sec-T1-dataAcquisition}

We collected multi-document legal case summarization data with 1,393 legal case samples from a widely recognized legal repository, Clearinghouse.
% \lu{do you crawl from the website or obtained through API? details here} 
We obtained the case data through the official Clearinghouse API\footnote{\url{https://clearinghouse.net/api}}, which provides structured access to metadata and associated documents for civil rights litigation cases. For documents available in PDF format, we used the ocrmypdf\footnote{\url{https://github.com/ocrmypdf/OCRmyPDF}} tool to extract text from scanned legal filings, ensuring complete retrieval of document content.
Each sample includes multiple case documents. Alongside these inputs, the dataset provides expert-crafted, gold-standard summaries that distill the key facts, legal principles, and outcomes of each case. These summaries are produced by trained legal experts—including lawyers and law students—who follow detailed annotation guidelines. To further ensure consistency and accuracy, each summary undergoes an additional round of expert review.
% \lu{who's the `expert'? law school undergrad and master and doctoral students?} 
% Each case document is available in both PDF and text formats.
% This rich and diverse dataset offers a valuable resource for studying the challenges of legal case summarization and evaluating the performance of large language models on complex, expert-level tasks.
We then selected a small, high-quality and representative subset from the large-scale dataset to evaluate the ability of LLMs in generating legal summaries. 

Concretely, for representative data selection, we filter the data based on the following standards to select a high-quality dataset.
\begin{itemize}
    \item \textbf{Diversity}: We obtain the topic for each case on the Clearinghouse website and select cases spanning as many distinct topics as possible. The selected data covers diverse case types such as "Equal Employment", "Prison Conditions", "Election/Voting Rights" which contain the specific topic the legal case is dealing with. \jie{will add the specific types num and threshold for difficulty factors}
    \item \textbf{Difficulty}: We identify several factors influencing difficulty through after discussing with legal researchers. The factors are as follows:
    \begin{itemize}
        \item \textbf{Length of the documents}: length of the documents is calculated by the total length of the case documents.
        \item \textbf{Number of appeals}: appeals are processes that the litigant asks for the higher court review of the lower court's decision, we obtain the number of appeals for each case on the clearinghouse website.
        \item \textbf{Number of complaints}: complaints are documents that start the lawsuit. We obtain the number of complaints for each case on the Clearinghouse website.
        \item \textbf{Number of dockets}: dockets are logs containing a comprehensive history of the case in chronological order. We obtain the number of dockets for each case on the clearinghouse website.
    \end{itemize} 
\end{itemize}
% \begin{itemize}
%     \item \textbf{Diversity}: The case topics should be varied.
%     % \lu{what is case type? what are the values for it?}
%     \item \textbf{Difficulty}: We consider the
% total length of the case documents, number of dockets, number of appeals, and number of complaints to ensure balance in difficulty.
% % \lu{i don't think you mentioned what types of documents can be in the input, when you introduce the task, you can ask the input documents, can be appeals, complaints, ....}
% \end{itemize}

% \lu{can merge this paragraph with the previous bullet points? avoid repetition}
% For \textbf{diversity}, we obtain the topic for each case on the Clearinghouse website and select cases spanning as many distinct topics as possible. The selected data covers diverse case types such as "Equal Employment", "Prison Conditions", "Election/Voting Rights" which contain the specific topic the legal case is dealing with. \jie{will add the specific types num and threshold for difficulty factors}
% For \textbf{difficulty}, we identify several factors influencing difficulty through after discussing with legal researchers. The factors are as follows:

% \begin{itemize}
%     \item \textbf{Length of the documents}: length of the documents is calculated by the total length of the case documents.
%     \item \textbf{Number of appeals}: appeals are processes that the litigant asks for the higher court review of the lower court's decision, we obtain the number of appeals for each case on the clearinghouse website.
%     \item \textbf{Number of complaints}: complaints are documents that start the lawsuit. We obtain the number of complaints for each case on the Clearinghouse website.
%     \item \textbf{Number of dockets}: dockets are logs containing a comprehensive history of the case in chronological order. We obtain the number of dockets for each case on the clearinghouse website.
% \end{itemize} 

After this process, we select 454 samples with high difficulty level considering the above factors.

To further ensure the quality of the gold-standard case summary created by legal researchers, we discuss with legal researchers and identify some essential information items that need to be covered in the summary in all cases. We then use GPT-4o as a judge to assess whether the human-written reference summaries of cases cover the essential information items and select the cases with high-quality human summaries. The specific prompt used for accessing the reliability of human-written summary is
% \lu{there are two tables, can we use smaller font to fit into 1 table?}
shown in Table \ref{tab:T1-reliablity}. Based on the judgment results, we finally select \textbf{100 samples} with high-quality and long human reference summary.

\begin{table}[H]
\centering
\small
\begin{tcolorbox}[title=Task 1-Legal Case Summarization: Prompt for checking the quality of human-written references, colback=yellow!5]
Evaluate whether the given summary includes all the information listed in the checklist items.
For each checklist item, provide whether the item is fully addressed ("Yes" or "No") and a brief explanation or evidence supporting your evaluation.
Finally, provide an overall result summarizing whether all checklist items are covered in the given summary.
Provide the overall result after \#\#\#\#, eg \#\#\#\# Yes or \#\#\#\# No.

Given Summary: [REQUEST]

Checklist Items:

\begin{itemize}
    \item Filing Date
    \begin{itemize}
        \item Whether it contains the Date: yes/no
    \end{itemize}
    \item Cause of Action   
    \begin{itemize}
        \item Description: e.g., a statute (e.g., 42 USC 1983) or a case (e.g., Ex Parte Young)
        \item Whether it contains the information: yes/no
        \begin{itemize}
            \item yes: the summary clearly states the action information
            \item no: do not mention the action information
        \end{itemize}
    \end{itemize}
    \item Statutory or Constitutional Basis for the Case
    \begin{itemize}
        \item   Description: A case can either be based on a statute or a provision of the Constitution--i.e., a case will either claim that someone violated a statute, or violated the Constitution. For cases that have a constitutional basis, the summary should refer to the clause of the Constitution that was allegedly violated, as well as the amendment if applicable. So for example it would say "the plaintiffs alleged violations of the Fourteenth Amendment's Equal Protection Clause," or "the plaintiffs alleged violations of the Commerce Clause."
        \item Whether it claim that someone violated a statute or violated the Constitution: yes/no
        \item Whether it contains the statutory bases information or constitutional bases information: yes/no
        \begin{itemize}
            \item yes: contains the statutory bases or constitutional bases information
            \item no: do not contain any statutory basis or constitutional bases information
        \end{itemize}
    \end{itemize}

\item Remedy Sought 
\begin{itemize}
  \item  Description: e.g., declaratory judgment
  \item  Whether it contains the information: yes/no
\end{itemize}
\item Who are the parties (description, not name)?
\begin{itemize}
    \item Whether it contains the information: yes/no
    \begin{itemize}
        \item Whether it contains the plaintiff information
        \item Whether it contains the description of the defendants (usually based on their office/position if it's a government official): yes/no
    \end{itemize}
\end{itemize}
\item Type of Counsel
\begin{itemize}
    \item Description: type of counsel contains private, legal services, ACLU, etc.
    \item Whether it contains the information: yes/no
\end{itemize}
\item First and Last Name of Judge 
\begin{itemize}
    \item Description: Form: Judge John Smith. 
    % Find judge’s first names at http://www.fjc.gov/public/home.nsf/hisj 
    \item Whether the reference includes this information and the generated result also includes it, or the reference does not include this information and the generated result also does not include it: yes/no
\end{itemize}
\item Factual Basis of Case
\begin{itemize}
    \item Description:  
    Refers to the facts or evidence upon which the case is built. These facts are essential in the legal process and are used to support legal claims or decisions. It typically includes:
    1. Details of the relevant events: For example, what happened, when it happened, where it happened, and who was involved. 
    2. Evidence: Physical evidence, documentary records, witness testimonies, etc., that support these facts. 
    3. Background information: Context or explanatory facts that provide additional understanding. 
    In legal proceedings, the factual basis is crucial for determining the outcome of a case, as the judge or jury makes decisions based on the facts and the applicable legal principles.
    \item Whether it contains the information: yes/no
\end{itemize}
\end{itemize}
\end{tcolorbox}
\caption{
Task 1-Legal Case Summarization: Prompt for checking the quality of human-written references.\jie{will confirm whether we could change font size in appendix (have checked the writing instruction but could not find related information)}
% \lu{add period, make caption full sentences}\lu{is this only for human written summaries or also used for system evaluation? like LLM as a judge evaluating model responses?} % only for human written summaries 
}
\label{tab:T1-reliablity}
\end{table}

% \begin{table}[h]
% \centering
% \begin{tcolorbox}
% Checklist Items:
% \begin{itemize}

% \item Factual Basis of Case
% \begin{itemize}
%     \item Description:  
%     Refers to the facts or evidence upon which the case is built. These facts are essential in the legal process and are used to support legal claims or decisions. It typically includes:
%     1. Details of the relevant events: For example, what happened, when it happened, where it happened, and who was involved. 
%     2. Evidence: Physical evidence, documentary records, witness testimonies, etc., that support these facts. 
%     3. Background information: Context or explanatory facts that provide additional understanding. 
%     In legal proceedings, the factual basis is crucial for determining the outcome of a case, as the judge or jury makes decisions based on the facts and the applicable legal principles.
%     \item Whether it contains the information: yes/no
% \end{itemize}
  
% \end{itemize}

% \end{tcolorbox}
% \caption{Task 1-Legal Case Summarization: Prompt for checking the quality of human-written references (Continued).}
% \label{tab:T1-reliablity2}
% \end{table}




\subsubsection{Illustrative Example}
The sample input for the legal case summarization task is multiple case documents. The human-written reference output is an expert-curated case summary. An example is shown in Table \ref{tab:T1-example}. Since the content of the case documents is long, we only demonstrate the purpose and topic of each case document. We will release all samples. \jie{should we create a anonymous github or doc to share some samples for each task to the reviewers?}
As shown in Table \ref{tab:T1-example}, the sample presents input data consisting of multiple legal documents from a class-action lawsuit related to COVID-19 conditions in immigration detention facilities. The inputs include court filings such as status reports, motions, court orders, and objections. These documents center around health and safety concerns at the Mesa Verde Detention Facility and the Yuba County Jail during the pandemic.
The reference output is a human-written summary that condenses the key developments and legal arguments of the case into a coherent summary. It captures the plaintiffs' claims about unsafe detention conditions, the legal basis of the lawsuit, court decisions such as the granting of temporary restraining orders and preliminary injunctions, and procedural milestones such as appeals and mediation efforts.
% Detailed example information could be found in our public GitHub repository.  

\begin{table}[H]
\centering
\begin{tcolorbox}[title=Task 1-Legal Case Summarization: A Sample of Case Documents and Summary]

\textbf{Case Documents (Sample Input):} % 17534

\textbf{Case Document 1:}

\{
Case 3:20-cv-02731-VC, Document 407 — Defendants’ Joint Status Report re COVID-19 Testing at Mesa Verde; 
Topic: COVID-19 testing plans and a positive case at Mesa Verde Detention Facility
\}

\textbf{Case Document 2:}

\{
Case 3:20-cv-02731-VC, Document 40 — Plaintiffs’ Opposition to Motion to Stay in Light of Fraihat;
Topic: Argument against staying proceedings due to a related case (Fraihat v. ICE)
\}

\textbf{Case Document 3:}

\{
Case 3:20-cv-02731-VC, Document 658 — Plaintiffs’ Objections to Defendants’ Medical Plan;
Topic: Critique of Defendants' COVID-19 medical care plan for Mesa Verde
\}

\textbf{Case Document 4:}

\{
Case 3:20-cv-02731-VC, Document 595 — Court Order to Create Medical Plan;
Topic: Court mandates improvement in COVID-19 medical response
\}


\textbf{Case Document 5:}

\{
Case 3:20-cv-02731-VC, Document 922 — TRO re: COVID-19 Conditions at Yuba County Jail;
Topic: Temporary Restraining Order to protect detainees at Yuba County Jail
\}

\textbf{Case Document 6:}

\{
Case 3:20-cv-02731-VC, Document 1106 — Motion to Strike GEO’s Attempt to Modify Injunction;
Topic: Plaintiffs seek to strike GEO’s motion to change court-ordered safety restrictions\}

...

\textbf{Case Summary (Human-written References): }

"COVID-19 Summary: This is a class-action lawsuit brought on April 20, 2020, by seven individuals in immigration detention at the Mesa Verde Detention Facility (MVDF) and the Yuba County Jail (YCJ), seeking immediate release from unsafe conditions of the jail in light of the global coronavirus pandemic. The court granted the request for TRO on April 29, requiring ICE to provide information and access to detainees to facilitate a process of considering bail requests. On June 9, the court granted the motion for preliminary injunction and ordered the defendants to maintain the status quo while the case was pending. On August 5, the plaintiffs sought a TRO, claiming that the defendants' actions were insufficient and it was granted the next day. After the parties agreed to implement testing and other public safety protocols, the defendants filed a motion to dismiss and the plaintiffs responded with an amended class-action complaint. The court granted a second preliminary injunction on December 3, 2020, and a preliminary injunction related to a YCJ outbreak on January 6, 2021. The defendants appealed to the Ninth Circuit and the parties entered into mediation.

On April 20, 2020, seven noncitizens detained at the Mesa Verde Detention Facility (MVDF) and the Yuba County Jail (YCJ) filed this class-action lawsuit against Immigration and Customs Enforcement (ICE), seeking immediate release from what they said were unsafe jail conditions in light of the global coronavirus pandemic. Represented by the ACLU of Northern California and Southern California, the San Francisco Public Defender's Office, Lawyers; Committee for Civil Rights, and private attorneys, the plaintiffs brought this lawsuit as a habeas petition under 28 U.S.C. under 2241, and as a declaratory action under 42 U.S.C. 2201-02. They alleged that their detention violated the Administrative Procedure Act, and their First and Fifth Amendment rights by subjecting them to a serious risk of contracting COVID-19. The plaintiffs sought a declaratory judgment and injunctive relief for the release of detainees in order to maintain a number of detainees for social distancing and prohibition against placing plaintiff class members into solitary confinement as a means of achieving social distancing, as well as attorney fees. The case was filed in the U.S. District Court for the Northern District of California and initially assigned to Magistrate Judge Sallie Kim, then reassigned to Judge Vince Chhabria. Concurrent with the complaint, plaintiffs sought class certification and a temporary restraining order to release a sufficient number of putative class members in order to allow for social distancing. The proposed class consisted of all civil immigration detainees at Mesa Verde and YCJ, with two subclasses: the YCJ Subclass; and the Mesa Verde Subclass.
..."

\end{tcolorbox}
\caption{Task 1-Legal Case Summarization: A Sample of Case Documents and Corresponding Summary.}
\label{tab:T1-example}
\end{table}

\subsubsection{Evaluation Rubric}
We closely collaborated with legal researchers to design a checklist-based evaluation rubric to assess the helpfulness of legal case summaries. This rubric comprises 26 checklist items that capture key aspects to consider during the evaluation process. Some items are marked as 'if applicable', meaning they should only be considered when the case pertains to the corresponding checklist criteria. The detailed checklist items are listed as follows:

\begin{itemize}
\item \textbf{Filing Date}

\item \textbf{Class Action or Individual Plaintiffs?} (if applicable): If there are class action plaintiffs the summary should say it's a class action; if there are individual plaintiffs it can just describe the plaintiffs. For example, use specific terms like "The city" or "The parents" rather than general terms like "The defendant" or "The plaintiffs."

\item \textbf{Cause of Action}: e.g., a statute (e.g., 42 USC 1983) or a case (e.g., Ex Parte Young)

\item \textbf{Statutory or Constitutional Basis for the Case}: A case can either be based on a statute or a provision of the Constitution---i.e., a case will either claim that someone violated a statute, or violated the Constitution. For cases that have a constitutional basis, the summary should refer to the clause of the Constitution that was allegedly violated, as well as the amendment if applicable. For example it would say "the plaintiffs alleged violations of the Fourteenth Amendment's Equal Protection Clause," or "the plaintiffs alleged violations of the Commerce Clause."
\item \textbf{Remedy Sought}: e.g., declaratory judgment

\item \textbf{Who are the parties (description, not name)?}

\item \textbf{Type of Counsel}: type of counsel contains private, legal services, ACLU, etc.

\item \textbf{Consolidated Cases Noted} (if applicable)

\item \textbf{Related Cases listed by their case code number} (if applicable)

\item \textbf{Note important filings} (if applicable): Note important filings including motions for temporary restraining orders or preliminary injunctions, motions to dismiss, motions for summary judgment, etc. 

\item \textbf{All reported opinions cited with shortened Bluebook citation} (if applicable): For example, the summary could write “2020 WL 4218003” after the paragraph in which it discusses that opinion.  The summary does not need to include the case name, court, or date unless helpful—such as when  the summary cites an opinion from a different case. 

\item \textbf{First and Last Name of Judge}: Form: Judge John Smith. Find judge’s first names at http://www.fjc.gov/public/home.nsf/hisj 

\item \textbf{Significant Terms of Decrees} (if applicable): Significant terms means the substance of the decree or settlement. In a decree, the judge orders the defendants to do something; in a settlement, the defendants agree to do something. The significant terms would be what the defendants are ordered/agree to do. 

\item \textbf{Dates of All Decrees} (if applicable)

\item \textbf{How long decrees will last} (if applicable)

\item \textbf{Significant Terms of Settlement} (if applicable)

\item \textbf{Date of settlement} (if applicable)

\item \textbf{How long settlement will last} (if applicable)

\item \textbf{Whether the settlement is court-enforced or not
} (if applicable)

\item \textbf{Was there a monitor? Note the name of the monitor} (if applicable)

\item \textbf{Monitor's Reports} (if applicable): A monitor's report explains whether a defendant is complying with a court order, so people want to know which terms of the order are being complied with. For example, from this case: In February 2016, the monitor filed her first semi-annual report. The report stated that the payment to the plaintiffs and plaintiffs counsel was made; the requirement of hiring ADA Coordinators was nearly compliant; videophone installation is apparently compliant; free access to videophone, provision of qualified interpreters for unscheduled medical emergencies, and provision of qualified interpreters for disciplinary hearings were unclear; informational materials were partially compliant; the routine and situational reporting were difficult or partially noncompliant; and training was noncompliant.

\item \textbf{Appeal} (if applicable)

\item \textbf{Trials} (if applicable)

\item \textbf{Court rulings on any of the important filings} (if applicable): This category corresponds with the "important filings" category---so whenever an important filing is mentioned, people also want to know what the ruling on that filing was (if there is one)---e.g., whether the judge granted or denied a motion to dismiss. Generally these filings would be:
Motions to dismiss, 
Motions for summary judgment, 
Motions for a preliminary injunction or temporary restraining order, 
Motions for class certification, 
Motions for attorneys' fees, 
Amended complaints--these won't have rulings, so they should be in the "important filings" category but not the "rulings on to important filings" category, statements of interest--similar to above, there won't be rulings on these.

\item \textbf{Factual basis of case}: Refers to the facts or evidence upon which the case is built. These facts are essential in the legal process and are used to support legal claims or decisions. It typically includes:
1. Details of the relevant events---For example, what happened, when it happened, where it happened, and who was involved.  
2. Evidence – Physical evidence, documentary records, witness testimonies, etc., that support these facts.  
3. Background information---Context or explanatory facts that provide additional understanding.  
In legal proceedings, the factual basis is crucial for determining the outcome of a case, as the judge or jury makes decisions based on the facts and the applicable legal principles.

\item \textbf{Disputes over settlement enforcement} (if applicable)

\end{itemize}

\subsubsection{Checklist-Mapped Reference}
To better evaluate the ability of models for generating legal case summaries according to our carefully designed fine-grained rubric, we construct a checklist-mapped reference by extracting the content corresponding to each checklist item from the case summary using GPT-4o. An example checklist-mapped reference is shown in Table \ref{tab:T1-Checklist-mappedReference}-\ref{tab:T1-Checklist-mappedReference3}. Specifically, for each checklist item, we follow its formal definition and instruct the model to extract relevant information from the generated summary.

Specifically, we adopt role-playing strategy and prompt the model to extract crucial related information from the human-written reference summary as completely as possible and if no related information is mentioned in the legal case summary, the model should state none. To ensure the extraction process is both cost-efficient and reliable, we group checklist items based on the expected length of their outputs and feed each group into the same prompt. We finally group the 26 checklist items for this task into 5 groups. The extraction prompt structure is illustrated in Table \ref{tab:T1-checklist-mappedReference-prompt}. Due to space limitations, we will release the full list of prompts used for the remaining information items in our public GitHub repository. 



\begin{table}[H]
\centering
\begin{tcolorbox}[title=Task 1-Legal Case Summarization: Checklist-mapped reference]
\begin{itemize}

\item \textbf{Filing Date}: 04/20/2020

\item \textbf{Class Action or Individual Plaintiffs?} (if applicable): Class Action

\item \textbf{Cause of Action}: Habeas petition under 28 U.S.C. § 2241 and declaratory action under 42 U.S.C. § 2201-02

\item \textbf{Statutory or Constitutional Basis for the Case}: Violations of the Administrative Procedure Act, the First Amendment, and the Fifth Amendment's Due Process Clause

\item \textbf{Remedy Sought}: Declaratory judgment, injunctive relief, release of detainees, prohibition of solitary confinement for social distancing, attorney fees

\item \textbf{Who are the parties (description, not name)?}: Plaintiff: Seven noncitizens detained at Mesa Verde Detention Facility and Yuba County Jail, represented by the ACLU of Northern and Southern California, the San Francisco Public Defender’s Office, Lawyers’ Committee for Civil Rights, and private attorneys; Defendants: U.S. Immigration and Customs Enforcement (ICE) and GEO Group, the ICE contractor operating the facility

\item \textbf{Type of Counsel}: ACLU of Northern California and Southern California, San Francisco Public Defender’s Office, Lawyers’ Committee for Civil Rights, and private attorneys

\item \textbf{Consolidated Cases Noted} (if applicable): Yes, appeals were consolidated under Case Nos. 21-15195 and 21-15197

\item \textbf{Related Cases listed by their case code number} (if applicable): 21-15195; 21-15197

\item \textbf{Note important filings} (if applicable): Temporary Restraining Orders (April 29, August 6, December 23, 2020); Preliminary Injunctions (June 9, December 3, 2020; January 6, 2021); Motion for Class Certification (April 2020); Motion to Stay (April 25, 2020); Motion to Dismiss (September 21, 2020 and January 19, 2021); Amended Complaint (October 30, 2020); Motion to Modify Preliminary Injunction (March 27 and June 1, 2021); Motion for Final Settlement Approval (May 27, 2022). 

\item \textbf{All reported opinions cited with shortened Bluebook citation} (if applicable): 2020 WL 2059848; 2020 WL 3055449; 2020 WL 4554646

\item \textbf{First and Last Name of Judge}: Vince Chhabria 

\item \textbf{Significant Terms of Decrees} (if applicable): Defendants were ordered to provide weekly rapid-result COVID-19 tests to all detainees, restrict new intakes, reserve dorms for isolation of positive cases, enforce social distancing (spacing of beds), perform symptom checks, isolate and test symptomatic detainees, report positive cases to plaintiffs’ counsel, file weekly status reports, test all staff weekly and bar untested staff from entry, and create a written plan for monitoring and responding to medical needs of high-risk detainees. Additional orders required detailed communication access for class counsel and monitoring of outbreak response at both MVDF and YCJ.

\item \textbf{Dates of All Decrees} (if applicable): April 29, 2020 (TRO); June 9, 2020 (Preliminary Injunction); August 6, 2020 (TRO); December 3, 2020 (Second Preliminary Injunction); January 6, 2021 (Preliminary Injunction for YCJ); June 9, 2022 (Final Settlement Approval)

\item \textbf{How long decrees will last} (if applicable): Until the end of the outbreak (after there had been no new positive tests for 2 consecutive weeks)


\end{itemize}
\end{tcolorbox}
\caption{Task 1-Legal Case Summarization: Checklist-mapped reference.}
\label{tab:T1-Checklist-mappedReference}
\end{table}

\begin{table}[H]
\centering
\begin{tcolorbox}[title=Task 1-Legal Case Summarization: Checklist-mapped reference (continued: Page 2)]
\begin{itemize}
\item \textbf{Significant Terms of Decrees} (if applicable): Defendants were ordered to provide weekly rapid-result COVID-19 tests to all detainees, restrict new intakes, reserve dorms for isolation of positive cases, enforce social distancing (spacing of beds), perform symptom checks, isolate and test symptomatic detainees, report positive cases to plaintiffs’ counsel, file weekly status reports, test all staff weekly and bar untested staff from entry, and create a written plan for monitoring and responding to medical needs of high-risk detainees. Additional orders required detailed communication access for class counsel and monitoring of outbreak response at both MVDF and YCJ.

\item \textbf{Dates of All Decrees} (if applicable): April 29, 2020 (TRO); June 9, 2020 (Preliminary Injunction); August 6, 2020 (TRO); December 3, 2020 (Second Preliminary Injunction); January 6, 2021 (Preliminary Injunction for YCJ); June 9, 2022 (Final Settlement Approval)

\item \textbf{How long decrees will last} (if applicable): Until the end of the outbreak (after there had been no new positive tests for 2 consecutive weeks)

\item \textbf{Significant Terms of Settlement} (if applicable): The settlement included limitations on the government’s ability to re-detain individuals released during the lawsuit, temporary and ongoing population caps to ensure social distancing, testing and vaccination mandates for detainees and staff, release of medically vulnerable individuals, and compliance with CDC guidelines. The government agreed to pay \$4 million in attorneys’ fees and process a \$120,000 cost reimbursement. The court retained jurisdiction over enforcement of the settlement for three years, and formally dismissed the case with prejudice upon final approval on June 9, 2022.

\item \textbf{Date of settlement} (if applicable): June 9, 2022

\item \textbf{How long settlement will last} (if applicable): Three years

\item \textbf{Whether the settlement is court-enforced or not
} (if applicable): Yes

\item \textbf{Was there a monitor? Note the name of the monitor} (if applicable): N/A

\item \textbf{Monitor's Reports} (if applicable): The court required defendants to file daily and weekly status reports on COVID-19 testing, quarantine efforts, and medical care at the Mesa Verde Detention Facility and Yuba County Jail. For example, after the August 6 TRO, the defendants were ordered to file daily reports about the status of the facility and efforts to manage COVID-19 risk. Plaintiffs later cited defendants' noncompliance with the January 6 preliminary injunction in a status report, pointing to lack of accurate and timely information, unclean cells, and failures to follow quarantine protocols. The court required the defendants to provide testing information for each class member at YCJ going back to December 11, 2020.

\item \textbf{Appeal} (if applicable): Defendants appealed to the Ninth Circuit

\item \textbf{Trials} (if applicable): N/A

\item \textbf{Court rulings on any of the important filings} (if applicable): The court granted multiple temporary restraining orders and preliminary injunctions: April 29, 2020 (TRO); June 9, 2020 (preliminary injunction); August 6, 2020 (TRO); December 3, 2020 (second preliminary injunction); January 6, 2021 (converted TRO into preliminary injunction for YCJ). The court denied the defendants' April 25 motion to stay proceedings, and denied a May 27 request to end the bail process and vacate orders. Judge Chhabria denied the defendants' September 21, 2020, motion to dismiss as moot, allowing an amended complaint. On February 23, 2021, the court denied another motion to dismiss and motion to transfer. Judge Chhabria denied a further motion related to the Pekoske memo on March 16, 2021.



\end{itemize}
\end{tcolorbox}
\caption{Task 1-Legal Case Summarization: Checklist-mapped reference (continued: Page 2).}
\label{tab:T1-Checklist-mappedReference2}
\end{table}


\begin{table}[H]
\centering
\begin{tcolorbox}[title=Task 1-Legal Case Summarization: Checklist-mapped reference (continued: Page 3)]
\begin{itemize}


\item \textbf{Factual basis of case}: The case involves a class-action lawsuit filed on April 20, 2020, by seven noncitizens detained at the Mesa Verde Detention Facility (MVDF) and the Yuba County Jail (YCJ), who sought immediate release due to unsafe conditions during the COVID-19 pandemic. The plaintiffs, many with underlying health conditions, faced inadequate access to hygiene, testing, and social distancing, prompting a hunger strike. Evidence includes detainee experiences, documented facility conditions, positive COVID-19 tests, and responses by ICE and GEO Group, the facility operator. The lawsuit cited violations of the APA and constitutional rights under the First and Fifth Amendments, and was supported by legal advocacy groups including the ACLU and the San Francisco Public Defender's Office.

\item \textbf{Disputes over settlement enforcement} (if applicable): After a preliminary settlement was reached in January 2022 and approved in June 2022, the court retained jurisdiction over disputes relating to interpretation and enforcement for three years. The plaintiffs filed a status report noting noncompliance with the January 6 preliminary injunction, including inaccurate reporting, lack of clean cells, and improper quarantine procedures. The court partially granted plaintiffs’ request for relief by ordering testing data disclosure, while denying other parts. These enforcement disputes occurred prior to the final approval of the settlement.

\end{itemize}
\end{tcolorbox}
\caption{Task 1-Legal Case Summarization: Checklist-mapped reference (continued: Page 3).}
\label{tab:T1-Checklist-mappedReference3}
\end{table}



\begin{table}[H]
\centering
\begin{tcolorbox}[title=Task 1-Legal Case Summarization: Prompt for extracting checklist-mapped reference, colback = yellow!5]

You are assisting a lawyer in extracting key information from a legal case summary. Given a case summary, extract

\begin{enumerate}
    \item the filing date,
    \item the cause of action, including whether it refers to a statute (e.g., 42 USC 1983) or a case (e.g., Ex Parte Young),
    \item the statutory or constitutional basis for the case, including any relevant constitutional clauses and amendments if applicable. A case can either be based on a statute or a provision of the Constitution--i.e., a case will either claim that someone violated a statute, or violated the Constitution. For cases that have a constitutional basis, the summary should refer to the clause of the Constitution that was allegedly violated, as well as the amendment if applicable. For example it would say "the plaintiffs alleged violations of the Fourteenth Amendment's Equal Protection Clause," or "the plaintiffs alleged violations of the Commerce Clause.
    \item the remedy sought (e.g., declaratory judgment),
    \item the remedy sought (e.g., declaratory judgment),
    \item the type of counsel mentioned (such as private, legal services, ACLU, etc.)
    \item the first and last name of the judge involved in the case and provide the extracted information. If the summary only mentioned the last name of the judge, only state the last name. If the summary only mentioned the first name of the judge, only state the first name.
\end{enumerate} 
   
Extract crucial related information as completely as possible. If no related information is mentioned in the legal case summary, state "N/A"(as a string).

Provide the output in json format. All values must be strings. Do not output objects, arrays, or nested structures. Example Format:

\{

\qquad    "Filing Date": "MM/DD/YYYY",
    
\qquad    "Cause of Action": "Cause of action",
    
\qquad    "Statutory or Constitutional Basis for the Case": 
    
\qquad    "Statutory or constitutional basis for the case",

\qquad    "Remedy Sought": "Remedy sought",
    
\qquad    "Type of Counsel": "Type of counsel",
    
\qquad    "First and Last name of Judge": "Name of Judge"
    
\}

This is the case summary:

\end{tcolorbox}
\caption{Task 1-Legal Case Summarization: Prompt for extracting checklist-mapped reference. }
\label{tab:T1-checklist-mappedReference-prompt}
\end{table}


To assess the quality of the Checklist-mapped references, we selected an additional 30 difficult and diverse samples which is different from the main dataset from the original large dataset. We conducted a human evaluation to examine the faithfulness of the Checklist-mapped references for these samples. Additionally, we used Gemini and Claude to evaluate both the faithfulness and coverage of the references. \jie{will add human evaluation details, results, automatic evaluation prompt, model details, results and conclusion once finish}

\subsection{Task 2: Legal - Brief Writing} \sheza{@sheza}\jie{@jie} \amy{@amy}

\subsubsection{Task Definition}
Legal brief writing entails generating detailed, structured, and self-contained summaries from juvenile court hearing transcripts. These briefs are not conventional legal briefs for court filing but serve as comprehensive documentation that captures the full scope of a hearing—particularly in child welfare and termination of parental rights cases. The primary goal is to create notes that encapsulate every relevant fact, testimony, procedural element, and judicial ruling in a format that is readable and actionable for legal teams, researchers, or case managers. These briefs are derived from transcripts and must include exact quotes, proper attribution, and clear connections to legal standards. The output should be sufficiently thorough to stand alone, eliminating the need to reference the original transcript. A standardized format is followed, including sections such as Hearing Overview, Participant Details, Witness Testimony, Procedural History, and Judge’s Ruling.

\subsubsection{Task Significance}
Legal brief writing plays a vital role in improving clarity, consistency, and accessibility in the documentation of juvenile court proceedings. Hearings in child welfare cases often involve complex, emotionally charged, and procedurally intricate content that must be translated into reliable and legally grounded summaries. Manual note-taking can miss key details, vary in quality, or lack comprehensiveness. Automating or augmenting this process using language models addresses these challenges by generating detailed, consistent, and structured briefs that follow a legally-informed rubric. These briefs aid attorneys, social workers, and judges by distilling essential information, highlighting statutory grounds, and surfacing patterns in non-compliance or risk. They are especially crucial in overburdened child welfare systems, where timely and accurate information directly impacts case decisions and the well-being of children. In this tasks, transcripts are drawn from real juvenile court proceedings\sheza{@jie need the data source details}, and outputs are compared against a detailed rubric developed with legal experts to ensure both completeness and legal relevance.

\subsubsection{Data Acquisition and Preprocessing}

Experts provided us with 113 samples of transcripts. We filtered these to 100 samples by the metrics of \amy{update once results are out}. 

\subsubsection{Illustrative Example}
The sample input for this task consists of an Adjudication Transcripts that occurred in 2010. We have omitted personal information from the example, and will refer In this example, the patient is a 55-year-old female with multiple chronic comorbidities who presents to the emergency department with chest pain and elevated blood pressure. The reasoning provided showed a diagnosis of Hypertension, citing risk factors (e.g., advanced age, family history of cardiovascular disease) and symptomatologies (e.g., chest pain as a sign of suspected Hypertension).


\begin{table}[H]
\begin{tcolorbox}[title=Task 2 - Legal Statement of Fact Generation: Sample]

\textbf{Transcript (Sample Input):}

\vspace{0.5em}
\textbf{TABLE OF CONTENTS} \hfill Page \\
Wednesday, December 1, 2010 — At about 8:58 a.m.

\vspace{0.5em}
\textbf{WITNESSES: MOTHER} \hfill \textbf{PAGE} \\
Eliezer Melendez \\
\quad Direct Examination by Ms. Kimble \dotfill 6 \\
\quad Voir Dire by Mr. Stevens \dotfill 7 \\
\quad Continued Direct Examination by Ms. Kimble \dotfill 8 \\
\quad Cross-Examination by Mr. Stevens \dotfill 14 \\
\quad Cross-Examination by Mr. Webb \dotfill 33 \\
\quad Examination by The Court \dotfill 7 \\
\quad Recross-Examination by Mr. Stevens \dotfill 28

\vspace{0.5em}
Christine Wilson (Recalled) \\
\quad Direct Examination by Ms. Kimble \dotfill 30 \\
\quad Cross-Examination by Mr. Stevens \dotfill 32

\vspace{0.5em}
\textbf{WITNESSES: JUVENILE} \\
\quad Direct Examination by Mr. Stevens \dotfill 38

\vspace{1em}
\textbf{TRANSCRIPT OPENING} \\

\noindent\textbf{THE COURT:} The record may reflect we are present in the matter of Payton Wilson. This is file number 10-4457 NA. Present in the courtroom is Mr. Stevens on behalf of the minor child. Ms. Kimble is present on behalf of Mother, who is present. Ms. Lock is present, represented by Mr. Webb.

This is a continuation of an adjudication hearing continued from November 1st so that Ms. Kimble could obtain witnesses that were not available at that time.

\textbf{MS. KIMBLE:} Your Honor, I would call Eliezer Melendez to the stand.

\textbf{THE COURT:} Up here, sir.

\textbf{MR. MELENDEZ:} Good morning.

\textbf{THE COURT:} Good morning. Raise your right hand, please. Do you solemnly swear or affirm to tell the truth?

\vspace{1em}
\textbf{Sample output (Human-written reference):}

This case involves the termination of the parental rights of Donald Frick to his daughter, Payton Wilson (DOB 01/23/2010).  At the time of the trial court’s decision to terminate Mr. Frick’s parental rights, he had never been provided with a service plan or parenting time with his daughter.  He had participated in parenting classes and other services he sought out on his own, was living with his wife,1 and was eager to support his child.  Mr. Frick’s rights were terminated despite the fact that he had never been provided with services to work toward reunification. \nThe child was taken into the custody of the Department of Human Services (“DHS”) on September 10, 2010, after being brought to the emergency room with multiple unexplained fractures and irritated eyes. 9/10/10 Order Taking Custody. DHS filed a petition seeking removal of Payton based on allegations against her mother, Christine Wilson. Original Petition, 9/13/10. 


\end{tcolorbox}
\centering
\caption{Task 2 - Legal Statement of Fact Generation: Sample}
\label{tab:T2-example}
\end{table}


\subsubsection{Evaluation Rubric}
In Task 2, we worked with two domain experts and drafted through three iterations of the checklist through discussion. The detailed checklist items are listed as follows:
\begin{itemize}
    \item When DHHS first made contact with the family
    \item What caused DHHS to become involved
    \item Discrepancies between DHHS’ account of the initial incident and the parent’s account of the initial incident
    \item Anyone (parent, social worker, the judge, attorneys, etc.) discussed any challenges the parent faced when they were young
    \item Anyone (parent, social worker, the judge, attorneys, etc.) discussed any problems the parent currently faces
    \item Anyone (parent, social worker, the judge, attorneys, etc.) discussed the child’s special needs
    \item Anyone (parent, social worker, the judge, attorneys, etc.) discussed how the child(ren) is doing
    \item Anyone (parent, social worker, the judge, attorneys, etc.) commented on the child(ren)’s development
    \item Anyone (parent, social worker, the judge, attorneys, etc.) commented on the child(ren)’s interactions with the parent
    \item Child(ren) talked about their feelings or experience
    \item What the judge decided to do after each court event (e.g., adjudication order, dispositional ruling)
    \item Anything new the parent or the child welfare agency (e.g., DHHS) has to do after each court event (e.g., adjudication order, dispositional ruling)
    \item Anything the parent or the child welfare agency (DHHS) does not have to do anymore after each court event (e.g., adjudication order, dispositional ruling)
    \item Whether the child welfare agency was ordered to make reasonable efforts to reunify
    \item If the agency was not ordered to make reasonable efforts to reunify, did it identify what aggravating circumstances were present
    \item Services the court required the parent to complete in the transcripts
    \item For each service, did it describe what the service means and what objectives the parents have to meet based on the transcripts
    \item Anyone (parent, social worker, the judge, attorneys, etc.) discussed how the parent participated in, did well, or complied with the services required
    \item Anyone (parent, social worker, the judge, attorneys, etc.) discussed how the parent did not participate or did not follow through with the services required
    \item Details on a parent’s compliance or noncompliance with the service plan
    \item Anyone (parent, social worker, the judge, attorneys, etc.) discussed how the child welfare agency tried to help the parent get the services they need
    \item Anyone (parent, social worker, the judge, attorneys, etc.) discussed how the agency or government might have ignored a parent or undermined their efforts
    \item When the adjudication hearing was held
    \item An adjudication trial or the parent pled to adjudication
    \item If the parent pled to adjudication, whether the statement identifies the specific allegations the parent pled to
    \item If there was an adjudication trial, whether the statement identifies what statutory grounds for adjudication the court found
    \item When each permanency planning hearing was held
    \item What permanency plan was established (e.g., reunification, adoption, guardianship etc.) at each permanency planning hearing
    \item Court’s reasons for the chosen permanency plan at each permanency planning hearing
    \item Whether DHHS was ordered to initiate termination of parental rights at each permanency planning hearing
    \item If the child has been in foster care for more than 15 of the last 22 months, and the court did not order DHHS to initiate termination proceedings, whether the statement identifies the court’s reasoning
    \item Under which statutory grounds DHHS sought termination
    \item Under which statutory grounds the court found that termination was proper
    \item Evidence that the parent offered to show statutory grounds for termination were not met
    \item Evidence the state offered to show termination was in the child’s best interests
    \item Evidence that the parent offered to show termination was not in the child’s best interests
    \item If the child was placed with a relative, whether any parties discussed that placement weighing against termination
    \item Evidence offered by the state regarding what kind of permanency (such as custody, adoption, or guardianship) the child will have if the parent’s rights are terminated
    \item Discusses alternatives to termination of parental rights
    \item Ends with the final lower-court ruling (e.g., “The court terminated parental rights on [date].”)
\end{itemize}


        
\subsubsection{Checklist-Mapped Reference}


\subsection{Task 3: Material Science - Synthesis Explanation Generation } \shuyang{@Shuyang}

\subsection{Task 4: Education - Pedagogy Evaluation} \inderjeet{@inderjeet}

\subsection{Task 5: Education - Feedback Generation} \inderjeet{@inderjeet}


\subsection{Task 6: Healthcare -  Clinical Note Generation} \amy{@Amy}\sheza{@sheza}\jie{@jie}

\subsubsection{Task Definition}
Clinical note generation is the task of producing well-structured, accurate, and comprehensive SOAP notes based on patient-doctor dialogue during a clinical encounter \cite{wikipedia_soapnote}. SOAP notes are made up of \textbf{S}ubjective, \textbf{O}bjective, \textbf{A}ssessment, and \textbf{P}lan sections, and are the most common way to document patient interactions \cite{podder2023soap}. The objective is to generate accurate, structured, and clinically useful SOAP notes from unstructured patient-doctor dialogues. This would greatly reduce the clinician workload and enhance the quality of medical documentation. A sample SOAP note is shown in Figure \ref{tab:T6-example}. In using LLMs to perform this task, we input a the transcript of a conversation between a healthcare professional and patient. The task output is a SOAP note that includes the key information from the conversation. 

\subsubsection{Task Significance}
Clinical documentation plays an important role in effective, high-quality care. It supports accurate diagnoses and standardizes communication among healthcare providers. However, the generation of structured clinical notes is time-consuming and prone to human error. Given the demanding schedule of healthcare professionals, critical details may be misremembered or entered in inaccurately. Automating this process with LLMs can improve consistency and create more efficient workflows, reducing patient wait times and improving patient care. 

\subsubsection{Data Acquisition}
We use the ACI-Bench dataset, a benchmark for clinical note generation with 207 annotated clinical encounters. Each sample includes a transcript of a patient-doctor interaction and its corresponding SOAP structured note written by the doctor \cite{yim2023aci}. Transcripts were created using three methods: (1) a virtual assistant, in which the doctor had to use explicit terms (e.g. ``Hey Dragon show me the diabetes lab") during the visit; (2) a virtual scribe, automated or otherwise, which assisted in note creation without distracting in-person doctor-patient interactions; and (3) an ambient clinical intelligence (ACI), which created the transcript without interrupting natural conversation flow between the patient and physician.

From these 207 samples, we selected a final subset of 100 through these criteria.
\amy{not sure if we are done filtering out 100 samples yet.}
% To further ensure the quality of the gold-standard case summary created by legal expert, we discuss with legal experts and identify some essential information items that need to be covered in the summary in all cases. We then serve GPT-4o as a judge to judge whether the human reference summaries of cases cover the essential information items and select the cases with high-quality human summary. The specific prompt is shown in Table \ref{tab:T1-reliablity} and Table \ref{tab:T1-reliablity2}. Based on the judgment results, we finally select 100 samples with high-quality and long human reference summary.

\subsubsection{Illustrative Example}
An example for this task is shown in Table \ref{tab:T6-example}. The input is a transcript of a multi-turn dialogue between a physician and a male patient presenting with an upper respiratory infection, in the context of underlying conditions such as depression, type 2 diabetes, and hypertension. The conversation covers topics including the patient’s lifestyle, recent symptoms, and adherence to treatment. The corresponding human-written reference output is a SOAP note authored by the physician who assesses the patient's conditions, gives follow-up recommendations, and potential diagnostic evaluations.

\begin{table}[H]
\centering
\begin{tcolorbox}[title=Task 6-Clinical Note Generation: A Sample of a Transcript and SOAP Note]
\textbf{Transcript (Sample Input):} % D2N001
[0][doctor] hi , andrew . how are you ?

[1][patient] hey , good to see you .

[2][doctor] i'm doing well , i'm doing well .

[3][patient] good .

[4][doctor] so , i know the nurse told you about dax . i'd like to tell dax a little bit about you .

[5][patient] sure .

[6][doctor] uh , so , andrew is a 59-year-old male with a past medical history , significant for depression , type two diabetes , and hypertension who presents today with an upper respiratory infection . so , andrew , what's going on ?

[7][patient] yeah . we were doing a bit of work out in the yard in the last week or so and i started to feel really tired , was short of breath . um , we- we're not wearing masks as much at the end of the summer and i think i caught my first cold and i think it just got worse .

[8][doctor] okay . all right . um , now , have you had your covid vaccines ?

[9][patient] yeah , both .

[10][doctor] okay . all right . and , um , do you have any history of any seasonal allergies at all ?

[11][patient] none whatsoever .

[12][doctor] okay . all right . and when you say you're having some shortness of breath , did you feel short of breath walking around or at rest ?

[13][patient] uh , usually , it was lifting or carrying something . we were doing some landscaping , so i was carrying some heavy bags of soil and i , i got really winded . it really surprised me .

[14][doctor] okay . and are you coughing up anything ?

[15][patient] not yet , but i feel like that's next .

% [16][doctor] okay . and fevers ?

% [17][patient] uh , i felt a little warm, but i, i just thought it was because i was exerting myself .

% [18][doctor] okay. all right. and any other symptoms like muscle aches , joint pain , fatigue ?

% [19][patient] my elbows hurt quite a bit and my knees were pretty tired . l- like i said , i really felt some tension around my knees , but , uh , i think that was a lot to do with , uh , lifting the bags .

% [20][doctor] okay . all right . um , so , you know , how about , how are you doing in terms of your other medical problems , like your depression ? how are you doing with that ? i know we've , you know , talked about not putting you on medication for it because you're on medication for other things . what's going on ?

% [21][patient] i- it's been kind of a crazy year and a half . i was a little concerned about that but , for the most part , i've been , been doing well with it . my , my wife got me into barre classes , to help me relax and i think it's working .

% [22][doctor] okay . all right , great . and , and in terms of your diabetes , how are you doing watching your , your diet and your sugar intake ?

...


\textbf{SOAP Note(Human-written Reference): }

\textbf{CHIEF COMPLAINT}\\
Upper respiratory infection.

\vspace{1em}

\textbf{HISTORY OF PRESENT ILLNESS}\\
Andrew Campbell is a 59-year-old male with a past medical history significant for depression, type 2 diabetes, and hypertension. He presents today with an upper respiratory infection.\\

The patient reports that he has been doing a bit of work out in the yard in the last week or so. He started to feel really tired and short of breath. The patient denies coughing up anything, but he feels like he will soon be coughing up phlegm. He denies having a fever, but he felt a little warm. He attributed this to exerting himself.\\

He reports that his elbows hurt quite a bit. He notes his knees were pretty tired and he felt some tension around his knees. The patient attributes these symptoms to lifting heavy bags. He has not been wearing a mask as much recently. He believes that he caught his first cold and his symptoms have worsened. He has had both of his COVID vaccinations.\\

He denies any history of seasonal allergies.\\

Regarding his depression, he states it has been a crazy year and a half. He was a little concerned about that, but for the most part, he has been doing well with it. His wife got him into barre classes and this has been relaxing.\\

Regarding his diabetes, he has been monitoring his sugar levels while he is at work, but is not as consistent on Saturdays and Sundays. His diet has been pretty good for the most part, except for some house parties. They have not been elevated since his respiratory symptoms began.\\
...
\end{tcolorbox}
\caption{Task 6-Clinical Note Generation: Sample of a Transcript and Corresponding SOAP Note}
\label{tab:T6-example}
\end{table}


\subsubsection{Evaluation Rubric}

In Task 6, we did not consult domain experts as in previous tasks, but created our rubric independently through extensive research. Our rubric items and definitions were verified across multiple reputable online sources \cite{wikipedia_soapnote} \cite{podder2023soap} and are still expert-level. The rubric comprises 28 checklist items that captures key information present in a SOAP note. The detailed checklist items are listed as follows:
\begin{itemize}
    \item \textbf{Reason for Patient Office Visit or Hospitalization:} Clearly states the primary reason for the patient's visit. Identifies the most pressing issue if multiple complaints are present.
    \item \textbf{Patient’s Age}
    \item \textbf{Patient’s Sex}
    \item \textbf{Patient’s Reason for the Visit}
    \item \textbf{Onset} (if applicable):  Clearly documents when the complaint started.
    \item \textbf{Location:} Specifies the exact location where the Chief Complaint happened.
    \item \textbf{Duration:} Indicates how long the complaint has persisted.
    \item \textbf{Character:} Describes how the patient describes the Chief Complaint.
    \item \textbf{Alleviating \& Aggravating Factors:} Lists what makes the Chief Complaint better or worse.
    \item \textbf{Radiation:} States whether symptoms move or stay localized.
    \item \textbf{Temporal Factor:} States if the complaint varies by time of day (e.g., worse in the morning).
    \item \textbf{Severity:} Patient's rating of the symptom on a scale from 1 to 10.
    \item \textbf{Relevant medical history: } Including past diagnoses, surgeries, and hospitalizations.
    \item \textbf{Surgical history }(if applicable)
    \item \textbf{Family history}
    \item \textbf{Home and Environment}
    \item \textbf{Education, Employment, Eating habits}
    \item \textbf{Activities}
    \item \textbf{Drugs}
    \item \textbf{Sexuality}
    \item \textbf{Suicide/Depression}
    \item \textbf{Other positive symptoms}
    \item \textbf{Other negative symptoms}
    \item \textbf{Vital Signs:} (e.g., BP, HR, RR, Temp, SpO2, weight, height if relevant). 
    \item \textbf{Physical Examination Findings: }including basic systems of cardiac and respiratory, the affected systems, possible involvement of other systems, pertinent normal findings and abnormalities. 
    \item \textbf{Other objective data} (if applicable): Results from laboratory and other diagnostic tests already completed.
    \item \textbf{Diagnosis \& Clinical Impression}: Provides a tentative diagnosis, assessment of patients status based on subjective and objective findings, a list of other possible diagnoses usually in order of most likely to least likely. The assessment will also include possible and likely etiologies of the patient's problem. It is the patient's progress since the last visit, and overall progress towards the patient's goal from the physician's perspective.
    \item \textbf{Treatment \& Management Plan}: The plan is what the health care provider will do to treat the patient's concerns—such as ordering further labs, radiological work up, referrals given, procedures performed, medications given and education provided. The plan will also include goals of therapy and patient-specific drug and disease-state monitoring parameters. This should address each item of the differential diagnosis. For patients who have multiple health problems that are addressed in the SOAP note, a plan is developed for each problem and is numbered accordingly based on severity and urgency for therapy. A note of what was discussed or advised with the patient as well as timings for further review or follow-up are generally included. This part is often grouped together with Assessment.
\end{itemize}

\subsubsection{Checklist-mapped Reference}
To better evaluate the ability of models to generate SOAP notes according to our carefully designed fine-grained rubric, we construct a checklist-mapped reference by extracting the content corresponding to each checklist item from the case summary using GPT-4o. Specifically, for each information item, we provide its formal definition and its corresponding section, and instruct the model to extract relevant information from the generated SOAP note.

\begin{table}[H]
\centering
\begin{tcolorbox}[title=Task 6-Clinical Note Generation: Prompt for extracting checklist-mapped reference]
 You are an experienced doctor reviewing clinical notes to identify key medical information. Given a clinical note, extract

 \begin{enumerate}
     \item the Reason for Patient Office Visit or Hospitalization information from the chief complaint in the subjective section. The Reason for Patient Office Visit or Hospitalization Clearly states the primary reason for the patient's visit. If multiple complaints are present, it identifies the most pressing issue.  
     \item the Patient’s Age information from the History of Present Illness in the subjective section.
     \item the Patient’s Sex information from the History of Present Illness in the subjective section.
     \item the Patient’s Reason information for the Visit from the History of Present Illness in the subjective section.
     \item the Onset information for the Visit from the History of Present Illness in the subjective section. The onset clearly documents when the complaint started.
     \item the Location information for the Visit from the History of Present Illness in the subjective section. The location specifies the exact location the Chief Complaint happened.
 \end{enumerate}
 
Extract crucial related information as completely as possible. If no related information is mentioned in the clinical note, state "N/A"(as a string). Provide the output in json format. All values must be strings. Do not output objects, arrays, or nested structures. Example Format:

\{

\qquad "Reason for Patient Office Visit or Hospitalization": "Reason for Patient Office Visit or Hospitalization",

\qquad "Patient Age": "Patient's Age",

\qquad "Patient Sex": "Patient's Sex",

\qquad "Patient Reason for the Visit": "Patient's Reason for the visit",

\qquad "Onset": "Onset",

\qquad "Location": "Location"

\}
   
    This is the clinical note:

\end{tcolorbox}
\caption{Task 6-Clinical Note Generation: Prompt for extracting checklist-mapped reference}
\label{tab:T6-checklist-mappedReference-prompt}
\end{table}

Specifically, we use a role-playing strategy and prompt the model to extract all relevant information as completely as possible. If a particular item is not mentioned in the SOAP note, the model is instructed to respond with ``N/A”. To ensure the extraction process is both cost-efficient and reliable, we group checklist items based on the expected length of their outputs and feed each group into the same prompt. We finally group the 28 checklist items for this task into 5 groups. The structure of the extraction prompt is shown in Table \ref{tab:T6-checklist-mappedReference-prompt}. Due to space constraints, we provide the complete set of prompts used for all information items in our public GitHub repository. An example checklist-mapped reference is shown in Table \ref{tab:T6-Checklist-mappedReference}.

\begin{table}[H]
    \begin{tcolorbox}[title=Task 6-Clinical Note Generation: Checklist-mapped reference]
    
\textbf{CHIEF COMPLAINT} \\
Upper respiratory infection. \\

\vspace{1em}
\textbf{HISTORY OF PRESENT ILLNESS} \\

\textbf{Patient's age, sex and reason for the visit:} Andrew Campbell is a 59-year-old male with a past medical history significant for depression, type 2 diabetes, and hypertension. He presents today with an upper respiratory infection. \\

\textbf{OLDCARTS:} The patient reports that he has been doing a bit of work out \textbf{[Location:]} in the yard \textbf{[Onset:]} in the last week or so. He started to feel really tired and short of breath. The patient denies coughing up anything, but he feels like he will soon be coughing up phlegm. He denies having a fever, but he felt a little warm. He attributed this to exerting himself. He reports that his elbows hurt quite a bit. He notes his knees were pretty tired and he felt some tension around his knees. The patient attributes these symptoms to lifting heavy bags. He has not been wearing a mask as much recently. \textbf{[Alleviating and Aggravating Factors:]} He believes that he caught his first cold and his symptoms have worsened. He has had both of his COVID vaccinations. \\

\textbf{[History:]} He denies any history of seasonal allergies. \\

\textbf{[Characterization:]} Regarding his depression, he states it has been a crazy year and a half. He was a little concerned about that, but for the most part, he has been doing well with it. \textbf{[Alleviating and Aggravating Factors:]} His wife got him into barre classes and this has been relaxing. \\

\textbf{[Radiation:]} Regarding his diabetes, he has been monitoring his sugar levels while he is at work, but is not as consistent on Saturdays and Sundays. His diet has been pretty good for the most part, except for some house parties. They have not been elevated since his respiratory symptoms began. \\

The patient has been monitoring his blood pressure at home. \textbf{[Temporal Factor:]} He reports that he is very regular with monitoring his blood pressure during the week, though less consistently on weekends. He reports his blood pressure has been under control. He has continued to utilize lisinopril 20 mg, daily. \\

The patient denies nausea, vomiting, diarrhea. \\

% \vspace{1em}
% \textbf{REVIEW OF SYSTEMS} 
% \begin{itemize}
%   \item \textbf{Constitutional:} Denies fever.
%   \item \textbf{Cardiovascular:} Endorses dyspnea on exertion.
%   \item \textbf{Respiratory:} Endorses shortness of breath and cough.
%   \item \textbf{Gastrointestinal:} Denies nausea or diarrhea.
%   \item \textbf{Musculoskeletal:} Endorses bilateral elbow and knee pain.
%   \item \textbf{Psychiatric:} Endorses depression.
% \end{itemize}

% \vspace{1em}
% \textbf{PHYSICAL EXAMINATION}
% \begin{itemize}
%   \item \textbf{Respiratory:} Scattered rhonchi bilaterally, clears with cough.
%   \item \textbf{Cardiovascular:} No murmurs, gallops, or rubs. No extra heart sounds.
%   \item \textbf{Musculoskeletal:} Edema in the bilateral lower extremities. Pain to palpation of the bilateral elbows.
% \end{itemize}
    \end{tcolorbox}
    \caption{Task 6-Clinical Note Generation: Checklist-mapped reference}
    \label{tab:T6-Checklist-mappedReference}
\end{table}

To assess the quality of the Checklist-mapped references, we selected an additional 30 difficult and diverse samples which is different from the main dataset from the original large dataset. We conducted a human evaluation to examine the faithfulness of the Checklist-mapped references for these samples. Additionally, we used Gemini and Claude to evaluate both the faithfulness and coverage of the references. \jie{will add human evaluation details, results, automatic evaluation prompt, model details, results and conclusion once finish}
% \begin{table}[H]
%     \begin{tcolorbox}

% \textbf{RESULTS} \\
% X-ray of the chest is unremarkable. No airspace disease. No signs of pneumonia. \\
% Hemoglobin A1c is elevated at 8. \\

% \vspace{1em}
% \textbf{ASSESSMENT AND PLAN} \\

% Andrew Campbell is a 59-year-old male with a past medical history significant for depression, type 2 diabetes, and hypertension. He presents today with an upper respiratory infection. \\

% \textbf{Upper respiratory infection} \\
% \begin{itemize}
%   \item \textbf{Medical Reasoning:} I believe he has contracted a viral syndrome. His chest x-ray was unremarkable and he has received both doses of the COVID-19 vaccination.
%   \item \textbf{Additional Testing:} We will obtain a COVID-19 test to rule this out.
%   \item \textbf{Medical Treatment:} I recommend he use Robitussin for cough, as well as ibuprofen or Tylenol if he develops a fever.
% \end{itemize}

% \textbf{Depression} \\
% \begin{itemize}
%   \item \textbf{Medical Reasoning:} He has been practicing barre classes and is doing well overall.
%   \item \textbf{Medical Treatment:} I offered medication or psychotherapy, but the patient opted to defer at this time.
% \end{itemize}

% \textbf{Diabetes type 2} \\
% \begin{itemize}
%   \item \textbf{Medical Reasoning:} His blood glucose levels have been well controlled based on home monitoring, but his recent hemoglobin A1c was elevated.
%   \item \textbf{Additional Testing:} We will repeat a hemoglobin A1c in 4 months.
%   \item \textbf{Medical Treatment:} We will increase his metformin to 1000 mg twice daily.
% \end{itemize}

% \textbf{Hypertension} \\
% \begin{itemize}
%   \item \textbf{Medical Reasoning:} He has been compliant with lisinopril and his blood pressures have been well controlled based on home monitoring.
%   \item \textbf{Additional Testing:} We will order a lipid panel.
%   \item \textbf{Medical Treatment:} He will continue on lisinopril 20 mg once daily. This was refilled today.
% \end{itemize}

% \textbf{Follow up:} I would like to see him back in approximately 4 months. \\
% \textbf{Patient Agreements:} The patient understands and agrees with the recommended medical treatment plan.


%     \end{tcolorbox}
%     \caption{Task 6-Clinical Note Generation: Checklist-mapped reference (continued: Page 2)}
%     \label{tab:T6-Checklist-mappedReference2}
% \end{table}


\subsection{Task 7: Chemistry -  Molecule Description} \amy{@Amy}\sheza{@sheza}\jie{@jie}

\subsubsection{Task Definition}
Molecule description generation is the task of creating accurate, structured, and human-readable descriptions of molecular structures based on their SMILES (Simplified Molecular Input Line Entry System) representations \cite{weininger1988smiles}. SMILES encodes molecules as linear strings that represent atoms, bonds, rings, and branching patterns, serving as a textual representation of molecular graphs. The objective is to translate these symbolic sequences into natural language descriptions that capture key structural and chemical features of the molecule. An example of an input-output pair is shown in Table \ref{tab:T7-example}. When applying LLMs to this task, the input consists of a SMILES string (e.g., CC(=O)OC1=CC=CC=C1C(=O)O). The output is a molecule description a professional might read.

\subsubsection{Task Significance}
Chemical databases contain tens of millions of molecules, each represented by complex SMILES strings that are not easily interpretable by humans. Experts find it time-consuming to understand the functional class or properties of a molecule from its SMILES representation, especially with more complex sequences. Automating the translation of SMILES into structured, ontological descriptions can enhance the accessibility and usability of chemical data, aiding in tasks such as drug discovery, materials science, and chemical education \cite{edwards2021text2mol}.

\subsubsection{Data Acquisition}

We utilize the ChEBI-20 dataset \footnote{\url{https://www.ebi.ac.uk/chebi/}}, which consists molecule-description pairs curated for training and evaluating models on this task. Each sample includes a SMILES string and its corresponding description. We then selected a small subset from this dataset to evaluate the ability of LLMs in generating molecule descriptions. We filter the data based on length and chose 224 samples with lengths greater than 500 characters.

To further ensure the quality of the gold-standard case summary created from CheBI, we discussed with chemistry experts to identify essential items that need to be covered in the molecule description. We then used GPT-4o as a judge to evaluate whether the human reference descriptions covered the information items and selected 100 descriptions with higher quality coverages. The specific prompt is shown in Table \ref{tab:T7-checklist-mappedReference-prompt}.
\amy{unsure about filtering process at the very end}

\subsubsection{Illustrative Example}
The sample input for the molecule description task is a general prompt curated by a domain expert and a SMILES string. We design in the prompt so that the task is defined in a high-level manner and rubric item definitions are not directly stated. An example is shown in Table \ref{tab:T7-example}.

In this example, the reference output is a description that summarizes the key chemical structure and pharmacological role of the molecule. It identifies the compound as alogliptin, a piperidine- and pyrimidine-based DPP-4 inhibitor used for the treatment of type 2 diabetes and highlights structural features such as the 2-cyanobenzyl and 3-aminopiperidinyl groups.

\begin{table}[H]
\centering
\begin{tcolorbox}
\textbf{SMILES string (Sample Input):} % D2N001

You are a chemical researcher in charge of writing descriptions of Chemicals of Biological significance given their Simplified Molecular Input Line Entry System (SMILES) structure. Use domain specific terminology and.specific molecule names. Be as specific as possible. Please provide your description in paragraph format. Here is the SMILES structure: ``CN1C(=O)C=C(N(C1=O)CC2=CC=CC=C2C\#N)N3CCC[C@H](C3)N"
\vspace{1 em}

\textbf{Molecule Description (Human-written Reference): }

The molecule is a piperidine that is 3-methyl-2,4-dioxo-3,4-dihydropyrimidine carrying additional 2-cyanobenzyl and 3-aminopiperidin-1-yl groups at positions 1 and 2 respectively (the R-enantiomer)\n Used in the form of its benzoate salt for treatment of type 2 diabetes\n It has a role as an EC 3\n4\n14\n5 (dipeptidyl-peptidase IV) inhibitor and a hypoglycemic agent\n It is a nitrile, a member of piperidines, a member of pyrimidines and a primary amino compound\n It is a conjugate base of an alogliptin(1+)\n\n

\end{tcolorbox}
\caption{Task 7-Clinical Note Generation: Sample}
\label{tab:T7-example}
\end{table}


\subsubsection{Evaluation Rubric}
Furthermore, we develop a fine-grained, checklist-based evaluation rubric in collaboration with a chemistry domain expert to ensure comprehensive coverage of key information for molecule. The expert not only advised us on the selection of rubric items, but also annotated a subset of human-written reference descriptions to identify which specific elements were explicitly or implicitly mentioned. These annotations informed the basis for the design of our checklist and guided the formulation of model prompts, ensuring that generated descriptions capture the same level of completeness and domain accuracy as the human references. The final rubric comprises six checklist items that captures key information present in a molecule description. The detailed checklist items are listed as follows:

\begin{itemize}
    \item \textbf{Structure:} The chemical composition of the molecule.
    \item \textbf{Biological Function and Applications:} The molecule’s functions in living organisms, including its interactions, effects on biological processes, and applications in the pharmacological domain.
    \item \textbf{Chemical compound classifications: }The specific group(s) of atoms that are used to categorize chemical compounds based on their structural characteristics, functional groups, or biological origin. 
    \item \textbf{Conjugate base} (if applicable): The species that remains after an acid donates a proton (H$^{+}$) in a chemical reaction. Usually, but not always, this description begins with “It is a conjugate base of”.
    \item \textbf{Conjugate acid} (if applicable): The species that remains after an base accepts a proton (H$^{+}$) in a chemical reaction. Usually, but not always, this description begins with “It is a conjugate acid of”.
    \item \textbf{Origin} (if applicable): The molecule or chemical compound that has been extracted or obtained from a specific natural resource.
\end{itemize}

\subsubsection{Checklist-mapped Reference}
To better evaluate the ability of models to generate descriptions according to our carefully designed fine-grained rubric, we construct a checklist-mapped reference by extracting the content corresponding to each checklist item from the case summary using GPT-4o. Specifically, for each information item, we follow its formal definition and instruct the model to extract relevant information from the generated summary.

We adopt a role-playing strategy and prompt the model to extract crucial related information as completely as possible. If no related information is mentioned in the molecule description, the model should state ``N/A". To ensure the extraction process is both cost-efficient and reliable, we group all six checklist items into one prompt. The extraction prompt is illustrated in Table \ref{tab:T7-checklist-mappedReference-prompt}. Due to space limitations, we will release the full list of prompts used for the remaining information items in our public GitHub repository. An example checklist-mapped reference is shown in Table \ref{tab:T7-Checklist-mappedReference}.


\begin{table}[H]
\centering
\begin{tcolorbox}[title=Task 7-Molecule Description Generation: Prompt for extracting checklist-mapped reference]
You are assisting a chemical researcher in extracting key information from a chemical molecule description. Given a description, extract its
 
 \begin{enumerate}
     \item Structure: the chemical composition of the molecule. Usually, but not always, this description begins with “The molecule is”.
    \item Biological function and applications: The molecule’s functions in living organisms, including its interactions, effects on biological processes, and applications in the pharmacological domain. Usually, but not always, this description begins with “It has a role as”.,
    \item Chemical compound classification: The specific group(s) of atoms that are used to categorize chemical compounds based on their structural characteristics, functional groups, or biological origin. Usually, but not always, this description begins with “It is a member of”.
    \item Conjugate base: The species that remains after an acid donates a proton (H$^{+}$) in a chemical reaction. Usually, but not always, this description begins with “It is a conjugate base of”.
    \item Conjugate acid: The species that remains after an base accepts a proton (H$^{+}$) in a chemical reaction. Usually, but not always, this description begins with “It is a conjugate acid of”.
    \item Origin: The specific natural resource the molecule has been extracted or obtained from. Usually, but not always, this description begins with “It is isolated from”.
 \end{enumerate}
    Extract crucial related information as completely as possible. If no related information is mentioned in the description, state "N/A"(as a string).
   
    Provide the output in json format. All values must be strings. Do not output objects, arrays, or nested structures. Example Format:
    
    \{
    
\qquad "Structure": "structure",

\qquad "Biological Function and Applications": "biological function and applications",

\qquad "chemical compound classifications": “chemical compound classifications”,

\qquad "Conjugate Acid": "conjugate acid",

\qquad "Conjugate Base": "conjugate base",

\qquad "Origin": “origin”
    
    \}
   
    This is the molecule description:
\end{tcolorbox}
\caption{Task 7-Molecule Description Generation: Prompt for extracting checklist-mapped reference}
\label{tab:T7-checklist-mappedReference-prompt}
\end{table}


\begin{table}[H]
    \begin{tcolorbox}[title=Task 7-Molecule Description Generation: Checklist-mapped reference]

    \begin{itemize}
    \item \textbf{Structure:} The molecule is a complex organic compound featuring multiple functional groups, including a nitrile, imidazole ring, and a conjugated system.
    \item \textbf{Biological Function and Applications:} It has a role as a potential bioactive compound, likely exhibiting pharmacological activity due to its intricate structure.
    \item \textbf{Chemical compound classifications: } It is a member of the class of heterocyclic compounds, specifically belonging to the subclass of imidazole derivatives, and includes a nitrile group and a benzene ring in its architecture. 
    \item \textbf{Conjugate base} (if applicable): N/A
    \item \textbf{Conjugate acid} (if applicable): It is a conjugate acid of the corresponding base where the nitrogen in the imidazole ring might accept a proton, enhancing its solubility and reactivity in biological systems.
    \item \textbf{Origin} (if applicable): N/A
\end{itemize}

    \end{tcolorbox}
    \caption{Task 7-Molecule Description Generation: Checklist-mapped reference}
    \label{tab:T7-Checklist-mappedReference}
\end{table}




\subsection{Task 8: Biology -  Protein Description} \amy{@Amy}\sheza{@sheza}\jie{@jie}

\subsubsection{Task Definition}
Protein description generation (or protein captioning) refers to generating an accurate, informative, and useful description of a protein given its amino acid sequence. These sequences are composed of letters representing individual amino acids and are the standard linear representations of protein primary structure. The objective is to generate a natural language description that captures essential biological characteristics of the protein, such as its function, cellular location, family or domain classification, and any relevant structural or catalytic properties. An example of a sequence-to-description pair is shown in Figure \ref{tab:T8-example}. In using LLMs to this task, the input is an amino acid sequence (e.g., MKWVTFISLLFLFSSAYSRGVFRRDTH...) and the model is prompted to output a protein description \cite{rives2021biological}.

\subsubsection{Task Significance}
Protein sequences are often long and complex, requiring expert knowledge and additional database lookups to understand their biological roles. Automatically generating informative descriptions from raw sequences makes protein data more accessible to biologists, students, and researchers working across molecular biology, genomics, and bioinformatics. This task has broad implications: it can support functional annotation in genome projects, improve interpretability in protein databases, and help build explainable AI systems for biological discovery \cite{li2023annopro}. By reducing the need for manual curation and facilitating faster insights into unknown or hypothetical proteins, automated protein captioning enhances biological research pipelines and educational tools alike.

\subsubsection{Data Acquisition and Preprocessing}
We collected protein sequences and their corresponding descriptions from the SciKnowEval dataset, which sources its protein-captioning entries from the UniProtKB database \footnote{\url{https://www.uniprot.org/help/uniprotkb}}—a comprehensive, curated resource for protein sequence and functional information \cite{feng2024sciknowevaleval}. Reference descriptions are written by experts and curated by UniProt and serve as the gold-standard for training and evaluation. From this dataset, we filtered a subset of 165 high-quality samples for our task. These samples were selected on length, all of which are over 900 characters. 

To further filter our dataset, we discussed with an expert in the biology domain and identified essential rubric items that are required to be covered in the description. We then use GPT-4o as a judge to evaluate whether the human reference descriptions cover this essential items and select the cases with highest-quality human references. The specific prompt is shown in Table \ref{tab:T8-Checklist-mappedReferencePrompt}. Based on these judgment results, we finally select 100 samples with high-quality and long human reference descriptions.

\subsubsection{Illustrative Example}
To guide the model in generating detailed and biologically relevant protein descriptions, we adopt a role-based prompting strategy. The model is instructed to assume the role of a professional protein researcher tasked with writing descriptions for protein sequences. The prompt encourages the use of domain-specific terminology. This example illustrates the specificity expected in generated descriptions. It captures functional roles (e.g., antimicrobial activity), cellular localization (extracellular), binding properties (lipopolysaccharide interaction), and structural features ($\beta$-strands with PDB references). 

\begin{table}[h]
\centering
\begin{tcolorbox}[title= Task 8-Protein Description Generation: Sample]
\textbf{Protein Sequence (Sample Input): 
}

You are a protein researcher in charge of writing descriptions of proteins given their sequence. Use domain specific terminology and specific molecule names. Be as specific as possible. Please provide your description in paragraph format. Here is the sequence: ``METQRASLCLGRWSLWLLLLGLVVPSASAQALSYREAVLRAVDRLNEQSSEANLYRLLELDQPPKADEDPGTPKPVSFTVKETVCPRPTRQPPELCDFKENGRVKQCVG\\TVTLDQIKDPLDITCNEVQGVRGGRLCYCRPRFCVCVGRG"\\

\textbf{Protein Description (Human-written Reference)}: 

This protein exhibits microbicidal activity and plays a crucial role in the antimicrobial humoral immune response mediated by antimicrobial peptides, defense against both Gram-negative and Gram-positive bacteria, and in the innate immune response. It is found in the extracellular space and has the ability to bind to lipopolysaccharides. It has a signal peptide that spans from amino acid 1 to 29, indicating it is directed outside the cell. Structurally, it contains beta-strands with evidence from PDB:2NC7, specifically in the regions from amino acids 135 to 139 and 142 to 146. This combination of functional, localization, and structural attributes, notably its role in immune responses, extracellular location, lipopolysaccharide-binding capacity, presence of a signal peptide, and beta-strand formation, makes it distinct within the protein universe.

\end{tcolorbox}
\caption{Task 8-Protein Description Generation: Sample}
\label{tab:T8-example}
\end{table}

\subsubsection{Evaluation Rubric}
We collaborated with two graduate students from the University of Michigan studying biology to create the evaluation rubric. We first presented an initial draft of the rubric and fine-tuned it with the experts' assistance across three separate meetings until both experts agreed with the rubric. The experts' also provided us with sources that explained their reasoning for including certain items in the rubric. They also consulted traditional protein caption characteristics, and ensured all aspects were present in the rubric. The rubric comprises ten checklist items that captures key information present in a protein description. The detailed checklist items are listed as follows:
\begin{itemize}
    \item \textbf{Primary Structure}: Amino acid sequence (e.g., 141 residues in $\alpha$-globin) \cite{berman2000protein} \cite{murzin1995scop}
    \item \textbf{Secondary Structure }(if applicable): Alpha-helices, beta-sheets, or loops. 
    \item \textbf{Tertiary Structure} (if applicable): 3D conformation (e.g., globular vs. fibrous).
    \item \textbf{Domains/Motifs}: Functional regions (e.g., kinase domain, zinc finger).
    \item \textbf{Functional Role}: How a molecule contributes to biological systems, including the processes it is involved in (e.g., metabolism, cellular functions) and the specific role it plays (e.g., enzymatic, structural, or signaling).\cite{szklarczyk2023string} \cite{oughtred2021biogrid}
    \item \textbf{Cellular Localization:} cellular location (e.g., mitochondrial matrix, cell membrane).
    \item \textbf{Gene Ontology:} Identify key GO terms. 
    \item \textbf{Clinical \& Biotech Relevance:} Role in diseases (e.g., amyloid-beta in Alzheimer’s), use as drug targets (e.g., insulin in diabetes), and applications in research and industry (e.g., Taq polymerase in PCR). \cite{wishart2018drugbank} \cite{anderson2015clinicaltrials} 
    \item \textbf{Interactions:} The physical and functional associations within a cell or organism, including but not limited to protein partners, ligands/substrates, and cofactors. 
\end{itemize}

\subsubsection{Checklist-mapped Reference}
To better evaluate the ability of models to generate descriptions according to our carefully designed fine-grained rubric, we construct a checklist-mapped reference by extracting the content corresponding to each checklist item from the description using GPT-4o. Specifically, for each information item, we follow its formal definition and instruct the model to extract relevant information from the generated summary.

If no related information is mentioned in the molecule description, the model should state ``N/A". To ensure the extraction process is both cost-efficient and reliable, we group all ten checklist items into two prompts based on category it extracts and length. The extraction prompt is illustrated in Table \ref{tab:T8-checklist-mappedReference-prompt}. Due to space limitations, we will release the full list of prompts used for the remaining information items in our public GitHub repository. An example checklist-mapped reference is shown in Table \ref{tab:T8-Checklist-mappedReference}.

\begin{table}[h]
\centering
\begin{tcolorbox}[title=Task8-Protein Description Generation: Checklist-mapped reference]

\begin{itemize}
    \item \textbf{Primary Structure}: It has a signal peptide that spans from amino acid 1 to 29, indicating it is directed outside the cell. 
    \item \textbf{Secondary Structure }(if applicable): Structurally, it contains beta-strands with evidence from PDB:2NC7, specifically in the regions from amino acids 135 to 139 and 142 to 146. 
    \item \textbf{Tertiary Structure} (if applicable): N/A
    \item \textbf{Domains/Motifs}: N/A
    \item \textbf{Functional Role}: This protein exhibits microbicidal activity and plays a crucial role in the antimicrobial humoral immune response mediated by antimicrobial peptides, defense against both Gram-negative and Gram-positive bacteria, and in the innate immune response. 
    \item \textbf{Cellular Localization:} It is found in the extracellular space
    \item \textbf{Gene Ontology:} N/A
    \item \textbf{Clinical \& Biotech Relevance:} N/A
    \item \textbf{Interactions:} and has the ability to bind to lipopolysaccharides. 
\end{itemize}

\end{tcolorbox}
\caption{Task8-Protein Description Generation: Checklist-mapped reference}
 \label{tab:T8-Checklist-mappedReference} 
\end{table}



\begin{table}[h]
\centering
\begin{tcolorbox}[title=Task 8-Protein Description Generation: Prompt for extracting checklist-mapped reference]
    You are assisting a protein researcher in extracting key information from a protein description. Given a description, extract its
    \begin{enumerate}
        \item Primary Structure: Amino acid sequence (e.g., 141 residues in $\alpha$-globin),
        \item Secondary Structure: Alpha-helices, beta-sheets, or loops.
        \item Tertiary Structure: 3D conformation (e.g., globular vs. fibrous).
        \item Domains and Motifs: Functional regions (e.g., kinase domain, zinc finger).
    \end{enumerate}

    Extract crucial related information as completely as possible. Extractions should come directly from the description in full sentence(s). If no related information is mentioned in the description, state ``N/A"(as a string).
   
    Provide the output in json format. All values must be strings. Do not output objects, arrays, or nested structures. Example Format:
    
    \{
    
\qquad "Primary Structure": "primary structure",

\qquad "Secondary Structure": "secondary structure",

\qquad “Tertiary Structure": “tertiary structure”,

\qquad “Domains and Motifs”: “domains and motifs”

    \}

    This is the protein description:
\end{tcolorbox}
\caption{Task8-Protein Description Generation: Prompt for extracting checklist-mapped reference \sheza{check placement later, right now it's showing up in task 9 text}}
 \label{tab:T8-Checklist-mappedReferencePrompt} 
\end{table}

% To evaluate the quality of the Checklist-mapped references, we selected an additional set of 30 challenging and diverse samples, distinct from the primary dataset. Human evaluators assessed the faithfulness of these references, ensuring they accurately reflected the source information. Furthermore, we employed advanced language models, Gemini and Claude, to assess both the faithfulness and coverage of the references. This dual evaluation approach provided a comprehensive understanding of the references' quality.


\subsection{Task 9: Medical - Discharge Summarization} \sheza{@Sheza}\jie{jie}

\subsubsection{Task Definition}
Medical discharge summarization involves creating a structured and comprehensive summary of a patient’s hospital stay, intended to support continuity of care and communicate key clinical information to healthcare professionals and patients. Data for this task are drawn from the MIMIC-IV database \cite{johnson2024mimic}, a large publicly available dataset of deidentified electronic health records (EHRs) from critical care units.

The \textbf{objective} is to generate an accurate and coherent discharge summary from structured and unstructured EHR data, which includes demographics, procedures, medications, diagnoses, laboratory results, vital signs, and clinical notes of the patient. The task simulates the workflow of physicians who synthesize these inputs into formal discharge documentation.

When applying language models to this task, the input consists of EHR data (structured fields and free-text clinical notes) from a single hospital admission, and the output is a physician-style discharge summary that encapsulates the entire episode of care. \jie{cite a sample figure/table here} Human reference summaries are those originally written by physicians in the MIMIC-IV-Note dataset \cite{johnson2023mimicnote}. These summaries serve as ground truth, reflecting expert synthesis of the relevant patient data.

While prior studies have used MIMIC datasets to explore text generation in the medical domain, existing work often emphasizes extractive summarization over complex long-form text generation or lacks detailed \jie{and finegrained} evaluation criteria. In contrast, our work utilizes the rich MIMIC-IV dataset, applying rigorous selection criteria and grounding the task definition in clinical documentation standards. We further extend this line of work by developing a checklist-based evaluation rubric derived from clinical best practices, specifically the Joint Commission’s discharge summary requirements \cite{kind2008documentation}, to assess the completeness and clinical relevance of generated outputs.

\subsubsection{Task Significance}
Discharge summaries are critical documents that ensure safe transitions of care, provide legal records of hospitalization, and facilitate communication between hospital teams, primary care providers, and patients. Poorly written or incomplete discharge summaries have been associated with adverse patient outcomes, such as medication errors, readmissions, and delayed follow-up care.

Automatically generating discharge summaries from EHR data can significantly reduce physician workload and documentation time, allowing clinicians to focus more on patient care. Language model-driven summarization can support more consistent and complete reporting, particularly in resource-constrained or high-throughput clinical settings.

This task advances the development of clinical language models by targeting a real-world, high-impact application that combines structured data reasoning and natural language generation. We introduce explicit selection criteria to ensure both \textbf{difficulty} and \textbf{diversity} in the dataset.\jie{add objective for data selection: selecte representative samples} Difficulty is determined through factors such as discharge summary length, number of admissions, ICU stay duration, and the complexity of diagnoses and procedures. Diversity is ensured across medication regimens, disease types, and patient demographics (age, gender, ethnicity). \jie{add where you get these meta-data, from the original database or somewhere else} By framing the task with robust data, expert references, and fine-grained evaluation, this work contributes to safer, more efficient, and more interpretable clinical AI systems.

\subsubsection{Data Acquisition and Preprocessing}

We compiled data using structured patient records and discharge summaries from the MIMIC-IV (v3.1) \cite{johnson2024mimic} and MIMIC-IV-Note (v2.2) \cite{johnson2023mimicnote} datasets, hosted on PhysioNet\footnote{\url{https://physionet.org/content/mimiciv/3.1/} and \url{https://www.physionet.org/content/mimic-iv-note/2.2/}}. These datasets provide large-scale, de-identified, real-world hospital data from the Beth Israel Deaconess Medical Center.

MIMIC-IV-Note contains 331,794 discharge summaries corresponding to 145,915 unique patients. Each summary contains long-form clinical narratives written by healthcare providers at the time of hospital discharge. In parallel, we used structured tables from MIMIC-IV to retrieve metadata and clinical signals related to the patient’s hospital stay, including diagnoses, procedures, ICU stays, and medications.

We then selected a small, high-quality and representative subset from the large-scale dataset to evaluate the ability of LLMs to summarize complex patient cases. 

For representative data selection, we filtered the data based on the following standards:

\begin{itemize}
    \item \textbf{Difficulty}: We identified several factors influencing medical case complexity based on clinical expert discussions and prior literature:
    \begin{itemize}
        \item \textbf{Length of the discharge summary}: We used token count as a proxy for textual complexity, prioritizing longer summaries.
        \item \textbf{Number of hospital admissions}: Frequent admissions may indicate chronic or recurring issues.
        \item \textbf{Length of ICU stay}: Prolonged ICU stays typically correlate with more critical cases.
        \item \textbf{Number of procedures and diagnoses}: A higher count of ICD codes indicates a more medically complex case.
    \end{itemize}
    
    \item \textbf{Diversity}: To ensure a representative and generalizable set of clinical conditions, we selected discharge summaries that varied across:
    \begin{itemize}
        \item \textbf{Medication diversity}: Patients prescribed a broader spectrum of drugs.
        \item \textbf{Disease diversity}: Based on diagnosis groupings (ICD-10 code variety).
        \item \textbf{Demographic attributes}: Age, gender, and ethnicity distributions.
    \end{itemize}
\end{itemize}

We first filtered the full dataset down to 10,898 discharge summaries using these criteria. From this filtered pool, we selected the top 120 most complex cases by ranking based on discharge summary length and validating that they met multiple difficulty and diversity factors. Each selected instance of human reference summary was linked to its structured records using shared identifiers (\texttt{subject\_id} and \texttt{hadm\_id}) and manually verified for completeness. The data filtering and preprocessing pipeline is implemented in Python \sheza{upload filter.ipynb on the project github}. 


\subsubsection{Illustrative Example}
The sample input for the discharge summary generation task consists of structured EHR data encompassing a patient’s hospital visit. This includes clinical information such as procedures, medications, diagnoses, laboratory results, vital signs, and physician notes. An example is shown in Table \ref{tab:T9-example}. Since the full EHR records are extensive, we only display a representative subset of the input data. As shown in Table \ref{tab:T9-example}, the sample presents detailed information from a single hospital admission, including procedure codes, medication orders, diagnostic labels, and lab test outcomes. The reference output is a physician-authored discharge summary that synthesizes this structured data into a coherent narrative. It summarizes key elements such as the hospital course, specialist consultations, performed procedures, discharge status, prescribed medications, as well as post-discharge instructions related to diet, activity, and follow-up care.

\begin{table}[H]
\centering
\begin{tcolorbox}[title=Task 9-Hospital Discharge Summary: A Sample EHR Record and Summary]

\textbf{Structured EHR Input (Sample Record):}


\textbf{Note ID:} 14767018-DS-20 \\
\textbf{Subject ID:} 14767018 \\
\textbf{HADM ID:} 21575486 \\
\textbf{Note Type:} DS (Discharge Summary) \\
\textbf{Chart Time:} 2156-07-27 00:00:00 \\
\textbf{Store Time:} 2156-07-27 21:46:00 \\
\textbf{Diagnoses (ICD-10)}  
\begin{itemize}
  \item Sepsis, unspecified organism (A419)
  \item Acute kidney failure with tubular necrosis (N170)
  \item Acute and subacute hepatic failure without coma (K7200)
  \item Acute respiratory distress syndrome (J80)
  \item Severe sepsis with septic shock (R6521)
  \item Pneumonia, unspecified organism (J189)
  \item Other sites of candidiasis (B3789)
  \item Chronic pulmonary edema (J811)
  \item Thrombosis due to vascular prosthetic devices, initial encounter (T82868A)
  \item Delirium due to known physiological condition (F05)...
\end{itemize} 
\textbf{Procedures (ICD-10-PCS)} 
\begin{itemize}
  \item Respiratory Ventilation, >96 Consecutive Hours (5A1955Z)
  \item Urinary Filtration, Multiple (5A1D60Z)
  \item Nutritional Substance to Upper GI, Via Opening (3E0G76Z)
  \item Infusion Device into Right Internal Jugular Vein (05HM33Z)
  \item Echocardiography (B543ZZA)*...
\end{itemize} 
\textbf{Drugs Administered} 
\begin{itemize}
  \item 5\% Dextrose (250 mL, IV)
  \item Heparin Sodium (25,000 unit Premix Bag, IV)...
\end{itemize} 
\textbf{Patient Summary (Human-written Reference):}\\
Name: \_\_\_ Unit No: \_\_\_ Admission Date: \_\_\_ Discharge Date: \_\_\_ Date of Birth: \_\_\_ Sex: F Service: MEDICINE\\
Allergies:
cefepime\\
Attending: \_\_\_.\\
Chief Complaint:
Acute hypoxemic respiratory failure\\
Major Surgical or Invasive Procedure:
intubation, bronchoscopy, extubation, LIJ, right tunneled HD line, HD\\
History of Present Illness:
Ms. \_\_\_ is a \_\_\_ year old woman with history of HTN, HLD, DM2 who presents from \_\_\_ with ARDS, acute liver injury, acute renal failure. According to her husband she was previously healthy, running half marathons, has had decline in health over past several years. She has had intermittent fatigue, joint pain, cough with intermittent paroxysmal episodes resulting in vomiting. She was being treated by a homeopathic healer for chronic lyme disease, taking at least 5 homeopathic medications. She has also had recurrent sinus infections, pneumonias. She was last treated for pneumonia Labor \_\_\_.  Patient initially presented \_\_\_ to \_\_\_ with complaints of weakness, lightheadedness, lower extremity edema. On presentation there she was found to have liver failure (reported transaminases in the thousands) and concern for obstructed biliary system. ERCP showed sludge. She underwent percutaneous cholecystostomy tube placement with concern for cholecystitis...\\
\end{tcolorbox}
\caption{Task 9-Hospital Discharge Summary: A Sample EHR Record and Corresponding Summary.\jie{describe what \_\_\_ mean}}
\label{tab:T9-example}
\end{table}


\subsubsection{Evaluation Rubric}
To evaluate the completeness and quality of discharge summaries, we designed a checklist-based evaluation rubric grounded in documentation standards published by the Joint Commission. Specifically, we follow the criteria outlined in the Joint Commission’s discharge summary content requirements, as detailed by Kind and Smith in their report on documentation quality during transitions from acute to subacute care \cite{kind2008documentation}.

This rubric consists of 12 checklist items that reflect the mandated components required for effective discharge communication. Several items are marked as 'if applicable', meaning they should be included only when clinically relevant to the patient’s case. The checklist enables standardized assessment of both the presence and quality of information in discharge documentation.

The full checklist items are as follows:

\begin{itemize} \item \textbf{Chief Complaint}: A clear statement identifying the primary reason for admission (e.g., “Patient admitted due to severe chest pain and shortness of breath”).

\item \textbf{History of Present Illness}: A concise summary of the patient’s presenting symptoms and their clinical progression (e.g., “A 58-year-old male with a history of hypertension presented with acute onset chest pain radiating to the left arm”).

\item \textbf{Primary Diagnosis}: The admission and discharge diagnoses should be explicitly documented (e.g., “Final diagnosis: Acute Myocardial Infarction”).

\item \textbf{Hospital Course}: A chronological overview of the clinical management and significant events during hospitalization (e.g., “Patient was started on heparin drip, underwent cardiac catheterization on Day 2”).

\item \textbf{Consultations} (if applicable): Documentation of any specialty consultations received (e.g., “Cardiology consult obtained for further evaluation of coronary artery disease”).

\item \textbf{Hospital Procedures} (if applicable): A list of diagnostic or therapeutic procedures conducted during the hospital stay (e.g., “Coronary angioplasty performed successfully”).

\item \textbf{Status at Discharge}: A brief statement describing the patient's condition at discharge (e.g., “Patient discharged in stable condition with no signs of distress”).

\item \textbf{Discharge Medications} (if applicable): A complete and updated list of prescribed medications upon discharge, including new, continued, and discontinued medications (e.g., “New prescriptions: Atorvastatin 40mg, Clopidogrel 75mg”).

\item \textbf{Activity Instructions} (if applicable): Specific recommendations or restrictions regarding physical activity (e.g., “Patient advised to avoid strenuous exercise for 2 weeks”).

\item \textbf{Therapy Orders} (if applicable): Instructions for physical, occupational, or speech therapy, if relevant (e.g., “Referral to outpatient cardiac rehab scheduled”).

\item \textbf{Dietary Instructions} (if applicable): Nutritional guidance tailored to the patient’s clinical condition (e.g., “Low-sodium, heart-healthy diet recommended”).

\item \textbf{Follow-up Appointments} (if applicable): Scheduled follow-up visits and provider contact details (e.g., “Follow-up with cardiologist in one week”). \end{itemize}

This evaluation framework ensures that discharge summaries are assessed for their alignment with clinical standards required for safe transitions of care and continuity across healthcare settings.

\subsubsection{Checklist-mapped Reference}
% example ref needs to be changed, this is an older one - setting as placeholder here

To assess model performance in generating discharge summaries aligned with critical clinical information needs, we construct checklist-mapped references that extract content corresponding to each checklist item from the original discharge summary using GPT-4o. An illustrative example of this process is shown in Table \ref{tab:T9-Checklist-mappedReference}. For each checklist item, we carefully follow its formal definition and prompt the model to extract the most relevant content from the discharge summary text.

Similar to our approach in Task 1, we adopt a role-playing prompt in which the model is instructed to act as a medical assistant tasked with extracting essential clinical information. If the information is not explicitly available in the summary, the model is instructed to return "N/A". To ensure efficiency and consistency, we group the checklist items based on content type and expected length, allowing multiple extractions within a single prompt. The example prompt used for this extraction is provided in Table \ref{tab:T9-checklist-mappedReference-prompt}.
\begin{table}[H] \centering \begin{tcolorbox}[title=Task 9-Hospital Discharge Summary: Checklist-mapped reference] \begin{itemize}

\item \textbf{Chief Complaint}: Transfer from OSH for HRS and liver transplant workup.

\item \textbf{History of Present Illness}: Mr. \underline{\hspace{3cm}} is a \underline{\hspace{3cm}} man with EtOH cirrhosis complicated by portal hypertension/ascites, history of subtotal colectomy for UC and colectomy for dysplasia/bleeding with post-op course complicated by decompensated portal hypertension, presenting with jaundice and pruritis. He had been doing well since his colectomy last year with ascites well controlled on diuretics. He began to experience itching several weeks before presentation. His family noticed jaundice and pruritis during a holiday visit, prompting him to see his PCP. Labs at the PCP visit showed elevated bilirubin (21) and creatinine (2.7). He was subsequently admitted to OSH and later transferred for further evaluation and liver transplant workup.

\item \textbf{Primary Diagnosis}: ETOH Cirrhosis, decompensated s/p liver transplant.

\item \textbf{Consultations}: Nephrology for renal failure and CRRT; Cardiology for atrial fibrillation and SVTs; Psychiatry for depression and delirium; Neurology for altered mental status; Infectious Disease for VRE bacteremia and MDR E. coli; Interventional Pulmonology for pleural effusions and empyema; Thoracic Surgery for empyema management; Geriatric Medicine for delirium management.

\item \textbf{Hospital Course}: The patient underwent a deceased donor liver transplant complicated by left rib fractures, takeback for re-exploration and control of bleeding, delayed abdominal closure with small bowel resection, diminished hepatic artery blood flow requiring splenic artery embolization, and biliary anastomotic stricture requiring ERCP and stent placement. His course was further complicated by altered mental status, cardiac arrhythmias (SVTs), persistent hypotension requiring pressors, respiratory failure with bilateral pleural effusions requiring chest tube drainage, multiple enterocutaneous fistulas, renal failure requiring CRRT/HD, hypothyroidism, adrenal insufficiency, and enterococcus bacteremia. He required multiple ICU admissions and extensive multidisciplinary care.

\item \textbf{Hospital Procedures}: Deceased donor liver transplant, re-exploration for bleeding, small bowel resection, splenic artery embolization, ERCP with stent placement, left thoracentesis, chest tube placements, right VATS pleural washout, percutaneous tracheostomy, right Eloesser flap, abdominal wound debridement, liver biopsy, and multiple abdominal washouts.

\item \textbf{Status at Discharge}: Expired.

\item \textbf{Discharge Medications}: 1. Albuterol 0.083\% Neb Soln Q6H PRN, 2. Dextrose 50\% IV PRN, 3. Ganciclovir 60 mg IV post-HD, 4. Glucagon 1 mg IM PRN, 5. Glucose Gel 15 g PO PRN, 6. Heparin 5000 UNIT SC BID, 7. HYDROmorphone 0.125-0.25 mg IV PRN, 8. Hydromorphone Oral Solution 1 mg/mL Q4H PRN, 9. Ipratropium Bromide Neb Q6H PRN, 10. Ipratropium-Albuterol Neb Q6H, 11. MethylPREDNISolone 4 mg IV Q24H, 12. Midodrine 10 mg PO TID, 13. Mycophenolate Mofetil 1000 mg IV BID, 14. Neomycin-Polymyxin-Bacitracin PRN, 15. Pantoprazole 40 mg IV Q12H, 16. Sarna Lotion QID PRN, 17. Sodium Chloride Nasal Spray QID PRN, 18. Sodium Polystyrene Sulfonate 15 gm PO PRN, 19. Sulfameth/Trimethoprim SS 1 TAB PO DAILY, 20. Tacrolimus 0.5 mg and 1 mg PO BID, 21. TraZODone 50 mg PO QHS.

\item \textbf{Activity Orders}: Out of bed with assistance to chair or wheelchair. No driving if taking narcotic pain medications.

\item \textbf{Therapy Orders}: N/A

\item \textbf{Dietary Instructions}: Eat small frequent meals, supplement with Carnation Instant Breakfast or Ensure. Avoid direct sun exposure and drink enough fluids to keep urine light in color.

\item \textbf{Follow-up Appointments}: Follow up with the transplant clinic. Labwork to be drawn twice weekly as arranged by the transplant clinic.

\end{itemize} \end{tcolorbox} \caption{Task 9-Hospital Discharge Summary: Checklist-mapped reference.} \label{tab:T9-Checklist-mappedReference} \end{table}
\begin{table}[H]
\centering
\begin{tcolorbox}[title=Task 9 - Hospital Discharge Summary: Prompt for extracting checklist-mapped reference, colback = yellow!5]

You are a medical professional extracting key clinical information from a hospital discharge summary. Given a discharge summary, extract:

\begin{enumerate}
    \item \textbf{Chief Complaint} – The main reason the patient was admitted to the hospital. Include associated symptoms and context, such as “presented with,” “admitted for,” etc.
    
    \item \textbf{History of Present Illness} – The timeline and progression of symptoms before admission. Include relevant medical, surgical, family, or social history, allergies linked to the complaint, and any patient-reported events or treatments prior to admission.
    
    \item \textbf{Primary Diagnosis} – The primary diagnosis at both admission and discharge. Include confirmed diseases, conditions, or syndromes. If multiple diagnoses are mentioned, extract the most emphasized one.
    
    \item \textbf{Consultations} – Any specialist consults requested during the stay. Include the specialty (e.g., cardiology), reason for consult, and recommendations or findings.
    
    \item \textbf{Hospital Course} – A summary of the clinical course during the hospital stay, including major events, complications, tests, clinical exams, and medical decision-making.
    
    \item \textbf{Hospital Procedures} – Diagnostic, surgical, or therapeutic procedures conducted. Include names, purposes, and results if mentioned.
    
    \item \textbf{Status and Disposition at Discharge} – The patient’s condition at discharge: symptom resolution, clinical stability, functional status, or changes since admission.
    
    \item \textbf{Discharge Medications and Instructions} – Prescribed medications and instructions at discharge. Include drug names, dosages, routes (e.g., oral, IV), and frequencies (e.g., once daily, BID).
    
    \item \textbf{Activity Orders} – Any physical activity-related instructions, such as walking or lifting restrictions.
    
    \item \textbf{Therapy Orders} – Physical, occupational, or speech therapy recommended post-discharge, with specified goals if given.
    
    \item \textbf{Dietary Instructions} – Any dietary restrictions or advice, such as diabetic diets or food restrictions.
    
    \item \textbf{Follow-up Appointments} – Recommended follow-up visits including specialty, reason, and timing (e.g., “follow up with cardiology in 2 weeks”).
\end{enumerate}

Extract all fields as thoroughly as possible. If a field is missing or not mentioned, return "N/A" (as a string). Do not make assumptions beyond the text. 

\textbf{Output format (all values must be strings, no arrays or nested structures):}

\begin{verbatim}
{
  "Chief Complaint": "string",
  "History of Present Illness": "string",
  "Primary Diagnosis": "string",
  "Consultations": "string",
  "Hospital Course": "string",
  "Hospital Procedures": "string",
  "Status at Discharge": "string",
  "Discharge Medications": "string",
  "Activity Orders": "string",
  "Therapy Orders": "string",
  "Dietary Instructions": "string",
  "Follow-up Appointments": "string"
}
\end{verbatim}

This is the discharge summary:

\end{tcolorbox}
\caption{Task 9 - Hospital Discharge Summary: Prompt for extracting checklist-mapped reference.}
\label{tab:T9-checklist-mappedReference-prompt}
\end{table}

As part of our quality control process, we manually evaluated the checklist-mapped references from 30 challenging and diverse discharge summaries sampled from the broader dataset. Evaluators assessed the extractions for faithfulness to the source text, and we additionally used GPT-based models such as Gemini and Claude to perform automated assessments of faithfulness and coverage. \sheza{To be updated with human and model evaluation details, prompts, results, and conclusion.} \jie{we may not use GPT-based models such as Gemini and Claude to do automatic assessments of this task}


\subsection{Task 10: Medical -  Diagnosis and Reasoning} \amy{@Amy}\sheza{@sheza}\jie{@jie}

\subsubsection{Task Definition}
The diagnosis and reasoning task aims to assess a model's ability to infer a Primary Discharge Diagnosis (PDD) from parts of a SOAP note. The input consists of the following sections of a SOAP note: the chief complaint, history of present illness, past medical history, family history, physical exam, and pertinent results. Any explicit mentions of the PDD are manually removed. Given the input, the model must predict the correct diagnosis and provide reasoning based on textual evidence. The reasoning is structured as a dictionary: \{\textit{o}: [\textit{z, r, d}]\}. \textit{o} is the extracted observation from raw text, \textit{z} is the rationale (created by humans or LLM) to explain why an observation can be related to a diagnosis \textit{d}, \textit{r} is the section (from one of input1-6) of the clinical note where \textit{o} is extracted, and finally \textit{d} is the name of the diagnosis. An example shown in Table \ref{tab:T10-example}.

\subsubsection{Task Significance}
This task addresses a challenge in clinical decision-making: providing accurate diagnoses from patient information. Errors in diagnosis can delayed treatment or inappropriate care, with severe consequences for patient outcomes. Additionally, correct diagnosis' can also be a result from inaccurate reasoning chains which will subsequently affect the treatment prescribed. By evaluating LLMs models' ability to support diagnostic inference in a structured and interpretable way, this task contributes to improving medical safety and clinical decision support systems.

\subsubsection{Data Acquisition}

The DiReCT dataset consists of 511 de-identified discharge summaries \cite{wang2024direct}. In each note, specific sections relevant to the diagnostic process were extracted: chief complaint, history of present illness, past medical history, family history, physical exam, and pertinent results. To ensure high quality data, reasoning annotations were performed by nine licensed clinical physicians and verified for accuracy and completeness by three senior medical experts. Each  diagnosis is one of 25 disease categories across five high-level clinical domains. Details of our dataset is shown in Table \ref{}. \amy{insert a table showing diagnosis type and number of samples for each}

We then selected a small, high-quality and representative subset from the large-scale dataset using the following filters:
\begin{itemize}
    \item \textbf{Diversity}: There should be a variety of diagnosis' present in the final samples. We would like to select an equal number of samples from each type of diagnosis.
    \item \textbf{Difficulty}: Longer reasoning chains usually correlate with more complex tasks. 
\end{itemize}

Using these filters, we selected six samples from each diagnosis, with a total of 150 samples. Then, we selected the 100 samples with the longest human reference output.

\subsubsection{Illustrative Example}
The sample input for this task consists of a SOAP note with labeled sections of the chief complaint, history of present illness, past medical history, physical exam, and lab results. In this example, the patient is a 55-year-old female with multiple chronic comorbidities who presents to the emergency department with chest pain and elevated blood pressure. The reasoning provided showed a diagnosis of Hypertension, citing risk factors (e.g., advanced age, family history of cardiovascular disease) and symptomatologies (e.g., chest pain as a sign of suspected Hypertension).

\begin{table}[H]
\centering
\begin{tcolorbox}[title=Task 10 - Diagnosis and Reasoning: Sample]
\textbf{SOAP Note (Sample Input):} % D2N001

   \textbf{Chief Complaint} (input1):
   
    chest pain
   
    \textbf{History of Present Illness }(input2):
    
    The patient is a 55 year old female with nonobstructive CAD, PVD, atrial fibrillation not on Warfarin, tachy-brady syndrome s/p PPM placement, hypertension, hypothyroidism, hyponatremia thought to be from primary polydipsia, and recurrent UTIs who presented to the ED ,left sided chest pain radiating to the neck, and suprapubic discomfort.
    
    She closely monitors her BP at home and self medicates with varying doses of Losartan between zero and four tabs daily. She reports that her BP was more elevated than usual this morning and kept increasing despite her taking multiple doses of Losartan, reaching the 200s in the evening. She felt somewhat lightheaded and developed pain in the left side of her chest and neck. 
    
   ...
    
\textbf{Diagnosis and Reasoning (Human-written Reference): }
\begin{verbatim}
{
  "Hypertension",
  {
    "her BP was reaching the 200s": [
      "An elevation of BP(SBP >= 140mmHg or DBP >= 90mmHg)confirmed is 
      a diagnostic criteria of Hypertension.",
      "input2",
      "Hypertension"
    ],
    "Initial vital in ED was BP 172/80": [
      "An elevation of BP(SBP >= 140mmHg or DBP >= 90mmHg)confirmed is 
      a diagnostic criteria of Hypertension.",
      "input2",
      "Hypertension"
    ]
  }
}
\end{verbatim}
\end{tcolorbox}
\caption{Task 10 - Diagnosis and Reasoning: Sample}
\label{tab:T10-example}
\end{table}

\subsubsection{Evaluation Rubric}

In Task 10, we did not consult domain experts as in previous tasks, but created our rubric independently. The rubric comprises 3 main checklist items that is dependent on the size of the human reference. The detailed checklist items are listed as follows:
\begin{itemize}
    \item \textbf{Diagnosis}
    \item For each Reasoning, Evidence pair
    \begin{itemize}
        \item Evidence
        \item Reasoning is present
    \end{itemize}
\end{itemize}

\subsubsection{Checklist-mapped Reference}
A checklist-mapped reference was not necessary in task as the data as the human reference and model output were created in a way that was structured. 


\subsection{Task 11: ESG} \shuyang{@shuyang}

\subsection{Task 12: Cybersecurity} 
\inderjeet{@inderjeet} \amy{@Amy}

\subsubsection{Task Definition}
This task focuses on assessing the security of Large Language Model (LLM) agents in generating structured risk descriptions from execution traces involving interactions between the agent, a user, and the environment. Each interaction is analyzed to determine whether it leads to a risky outcome and, if so, why. The goal is to produce a binary safety label (0 if the execution trace is safe, and 1 if it is dangerous) and a detailed explanation of the risk. The explanation should contain all parts of a MTO (Motivation, Trigger, Outcome) schema \cite{yuan2024rjudge} and specify any trigger or attack tools. Definitions of these terms can be found in the Evaluation Rubric. 

\subsubsection{Task Significance}
LLM agents are increasingly deployed in interactive, real-world environments, where their actions can unintentionally introduce safety risks. These risks may lead to financial loss, data breaches, property damage, or other security threats. This task is critical for identifying such risks and understanding their origins, enabling the development of more secure and trustworthy autonomous agents.

\subsubsection{Data Acquisition and Preprocessing}
We first collected 108 samples from two execution trace datasets: AgentHarm and R-Judge. We selected 19 samples from AgentHarm and 81 samples from R-Judge. The following criteria was used to filter the data: 
\begin{itemize}
    \item Diversity: From AgentHarm, we wanted 
\end{itemize}

\begin{enumerate}
    \item \textbf{AgentHarm} was designed to measure the harmfulness of LLM agents by evaluating their responses to explicitly malicious tasks across 11 harm categories, including fraud, cybercrime, and harassment \cite{andriushchenko2024agentharm}. It contained execution traces, trigger tools, and attack tools, but no risk descriptions. \amy{I don't remember how this data was collected}
    \item \textbf{R-Judge}  comprises 569 records of multi-turn agent interactions, encompassing 27 key risk scenarios among 5 application categories and 10 risk types \cite{yuan2024rjudge}. It contained risk descriptions with following the MTO schema, but no 
\end{enumerate}


Human annotations were produced by six domain-informed annotators (1 PhD candidate, 3 master’s students, 2 senior undergraduates) with backgrounds in AI, computer science, and cybersecurity. 


Each sample includes detailed interaction traces, which were manually reviewed and annotated.

\subsubsection{Illustrative Example}


\subsubsection{Evaluation Rubric}



\subsubsection{Checklist-Mapped Reference}



\subsection{Task XX: Sample Task}
\sheza{copy subheadings from here for each task subsection}
\subsubsection{Task Definition}
\subsubsection{Task Significance}
\subsubsection{Data Acquisition and Preprocessing}
\subsubsection{Illustrative Example}
\subsubsection{Evaluation Rubric}
\subsubsection{Checklist-Mapped Reference}

\section{Breakdown Results on Different Disciplines}
